# Supplementary material for: Professor Preece's tredoku tilings
Source: arXiv:2511.12680 ancillary file (2025-11-16)
Supplement: Supplementary file 1 [file Appendix_A.pdf]

**Professor Preece's Tredoku Tilings**

## Appendix A - Extensions to tredoku tilings

This appendix shows all the extensions to tredoku tilings that appear in Donald's notes. There are 25 internal extensions and 3 external extensions.

### Internal Extension 1

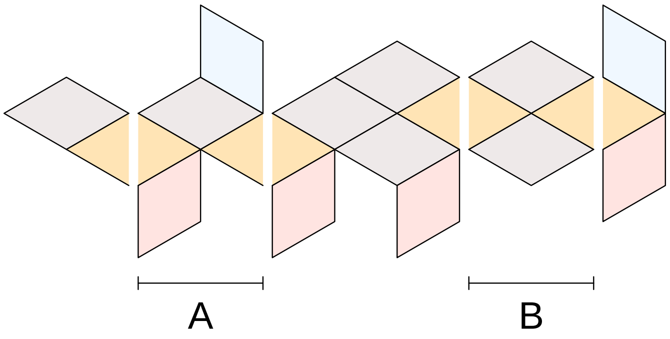


**Figure A1.** In this construction, segment A is repeated $a$ times ($a \geq 0$) and segment B is repeated $b$ times ($b \geq 1$), giving $\tau = 10 + 4a + 3b$ and $\rho = 5 + 2a + 2b$, so that $\tau = 2\rho - b$ for odd $\rho \geq 7$.

### Internal Extension 2

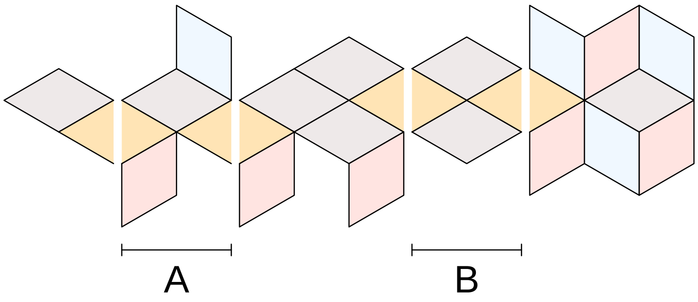


**Figure A2.** In this construction, segment A is repeated $a$ times ($a \geq 0$) and segment B is repeated $b$ times ($b \geq 1$), giving $\tau = 15 + 4a + 3b$ and $\rho = 9 + 2a + 2b$, so that $\tau = 2\rho - b - 3$ for odd $\rho \geq 11$.

## Internal Extension 3

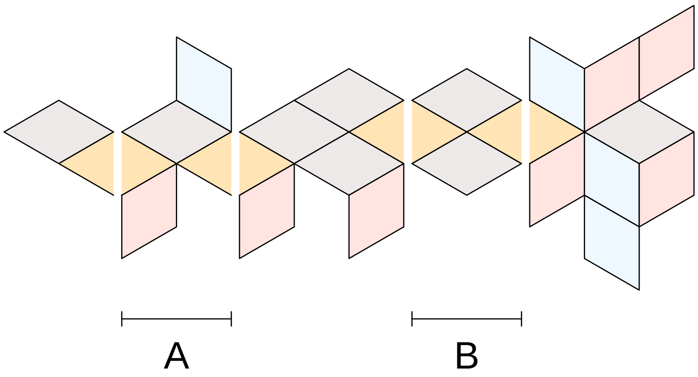


**Figure A3.** In this construction, segment A is repeated $a$ times ($a \geq 0$) and segment B is repeated $b$ times ($b \geq 1$), giving $\tau = 16 + 4a + 3b$ and $\rho = 9 + 2a + 2b$, so that $\tau = 2\rho - b - 2$ for odd $\rho \geq 11$.

## Internal Extension 4

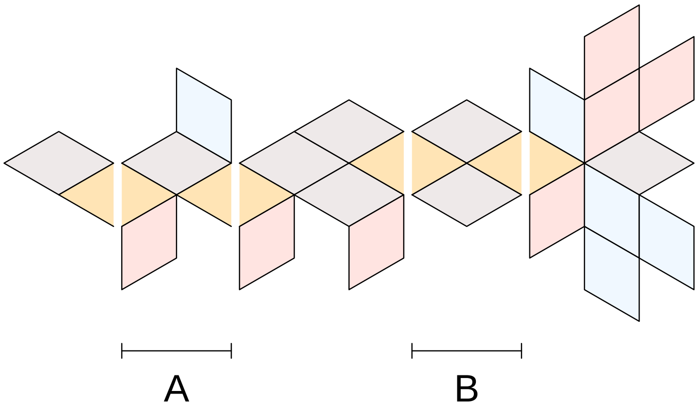


**Figure A4.** In this construction, segment A is repeated $a$ times ($a \geq 0$) and segment B is repeated $b$ times ($b \geq 1$), giving $\tau = 17 + 4a + 3b$ and $\rho = 9 + 2a + 2b$, so that $\tau = 2\rho - b - 1$ for odd $\rho \geq 11$.

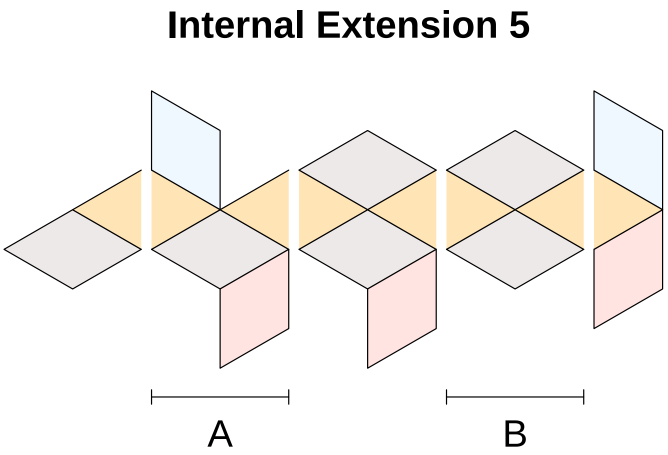


**Figure A5.** In this construction, segment A is repeated $a$ times ($a \geq 0$) and segment B is repeated $b$ times ($b \geq 1$), giving $\tau = 8 + 4a + 3b$ and $\rho = 4 + 2a + 2b$, so that $\tau = 2\rho - b$ for even $\rho \geq 6$.

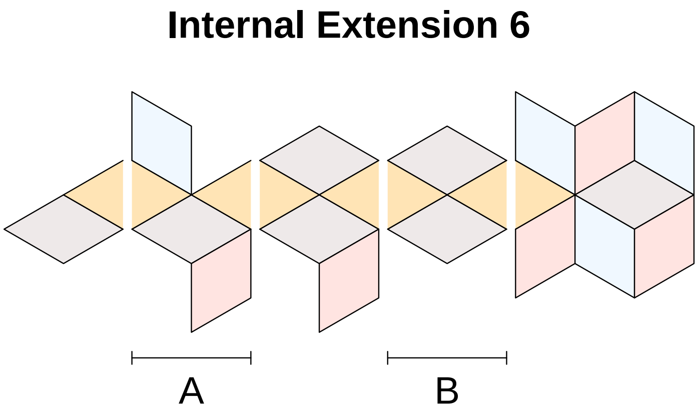


**Figure A6.** In this construction, segment A is repeated $a$ times ($a \geq 0$) and segment B is repeated $b$ times ($b \geq 1$), giving $\tau = 13 + 4a + 3b$ and $\rho = 8 + 2a + 2b$, so that $\tau = 2\rho - b - 3$ for even $\rho \geq 10$.

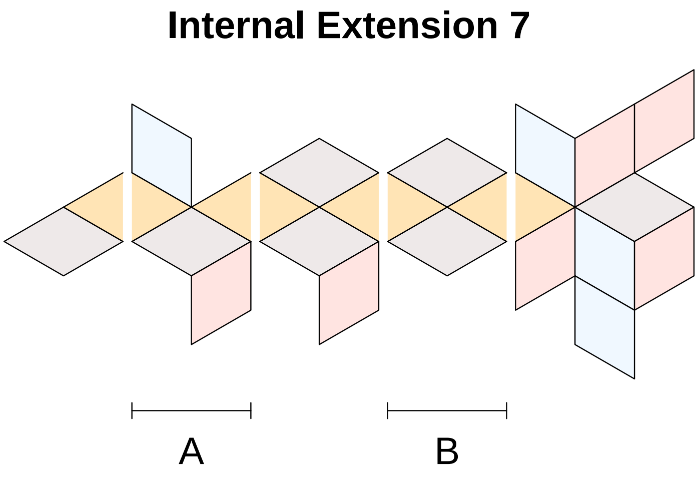


**Figure A7.** In this construction, segment A is repeated $a$ times ($a \geq 0$) and segment B is repeated $b$ times ($b \geq 1$), giving $\tau = 14 + 4a + 3b$ and $\rho = 8 + 2a + 2b$, so that $\tau = 2\rho - b - 2$ for even $\rho \geq 10$.

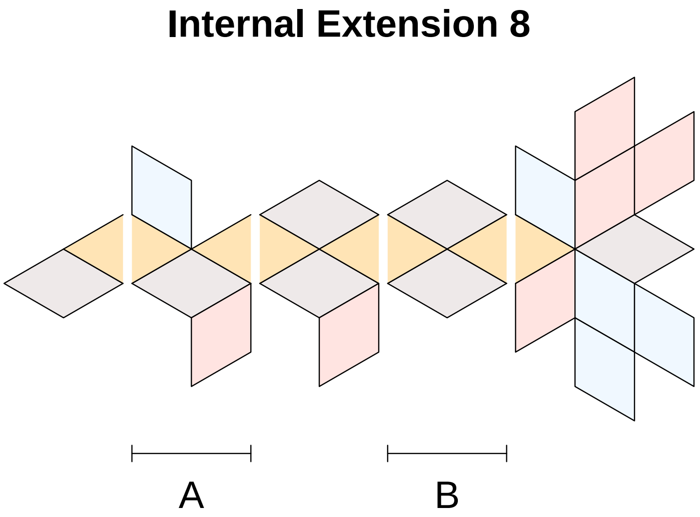


**Figure A8.** In this construction, segment A is repeated $a$ times ($a \geq 0$) and segment B is repeated $b$ times ($b \geq 1$), giving $\tau = 15 + 4a + 3b$ and $\rho = 8 + 2a + 2b$, so that $\tau = 2\rho - b - 1$ for even $\rho \geq 10$.

## Internal Extension 9

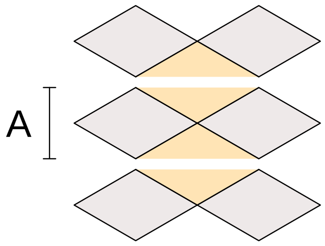


**Figure A9.** Construction 9 gives tilings with $\tau = (3\rho + 4)/2$ for even $\rho \geq 2$. Segment A is repeated $a$ times ($a \geq 0$), giving $\tau = 5 + 3a$ and $\rho = 2 + 2a$.

## Internal Extension 10

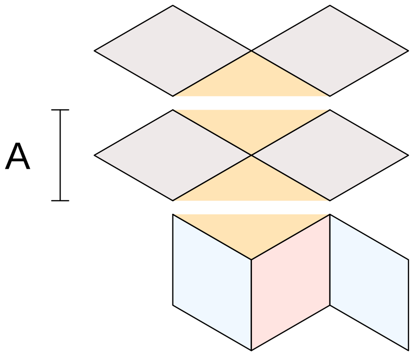


**Figure A10.** Construction 10 gives tilings with $\tau = (3\rho + 3)/2$ for odd $\rho \geq 3$. Segment A is repeated $a$ times ($a \geq 0$), giving $\tau = 6 + 3a$ and $\rho = 3 + 2a$.

## Internal Extension 11

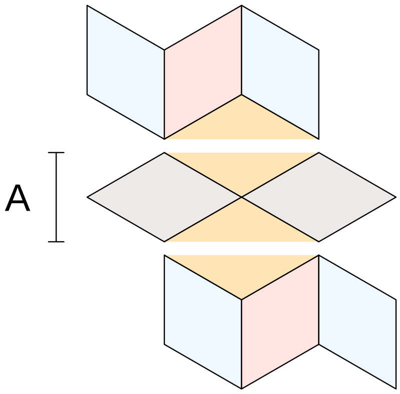


**Figure A11.** Construction 11 gives tilings with $\tau = (3\rho + 2)/2$ for even $\rho \geq 4$. Segment A is repeated $a$ times ($a \geq 0$), giving $\tau = 7 + 3a$ and $\rho = 4 + 2a$.

## Internal Extension 12

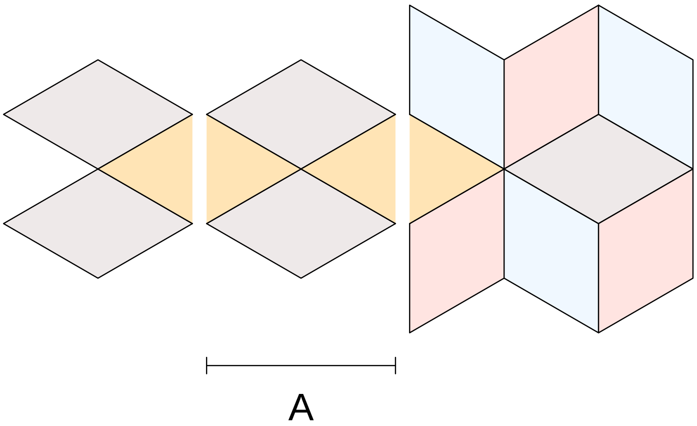


**Figure A12.** Construction 12 gives tilings with $\tau = (3\rho + 2)/2$ for even $\rho \geq 6$. Segment A is repeated $a$ times ($a \geq 0$), giving $\tau = 10 + 3a$ and $\rho = 6 + 2a$.

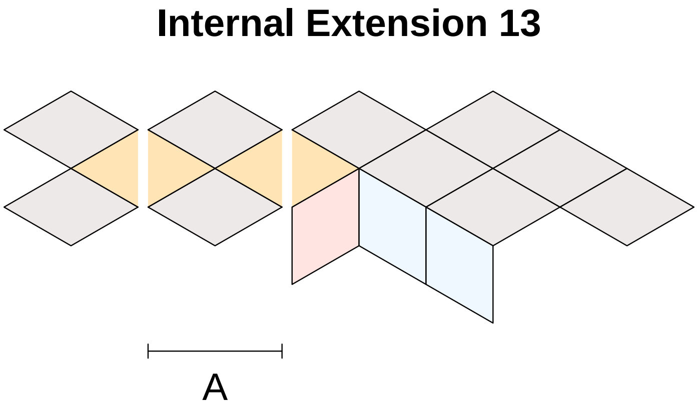


**Figure A13.** Construction 13 gives tilings with $\tau = (3\rho + 3)/2$ for odd $\rho \geq 7$. Segment A is repeated $a$ times ($a \geq 0$), giving $\tau = 12 + 3a$ and $\rho = 7 + 2a$.

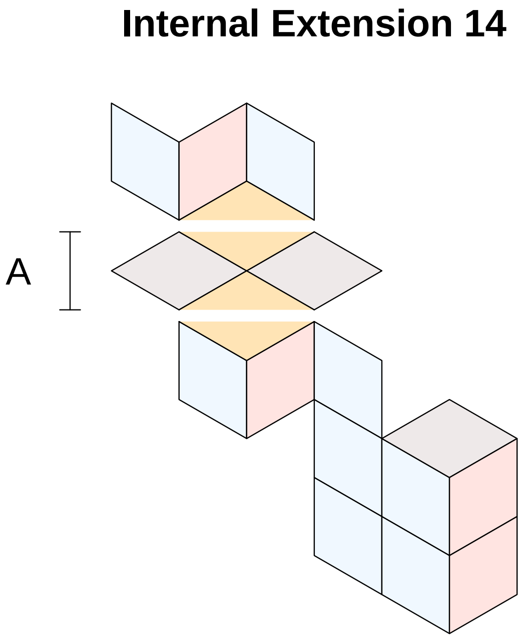


**Figure A14.** Construction 14 gives tilings with $\tau = (3\rho + 1)/2$ for odd $\rho \geq 9$. Segment A is repeated $a$ times ($a \geq 0$), giving $\tau = 14 + 3a$ and $\rho = 9 + 2a$.

## Internal Extension 15

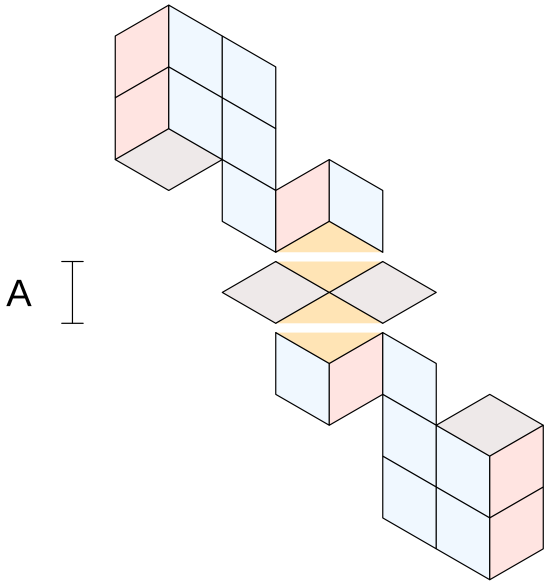


**Figure A15.** Construction 15 gives tilings with $\tau = 3\rho/2$ for even $\rho \geq 14$. Segment A is repeated $a$ times ($a \geq 0$), giving $\tau = 21 + 3a$ and $\rho = 14 + 2a$.

## Internal Extension 16

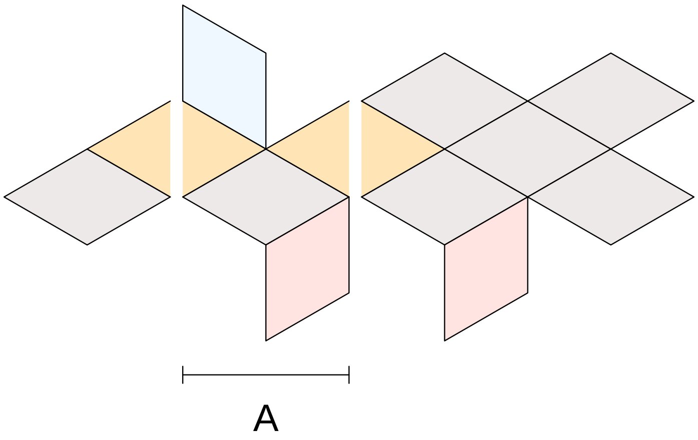


**Figure A16.** Construction 16 gives tilings with $\tau = 2\rho$ for even $\rho \geq 4$. Segment A is repeated $a$ times ($a \geq 0$), giving $\tau = 8 + 4a$ and $\rho = 4 + 2a$.

## Internal Extension 17

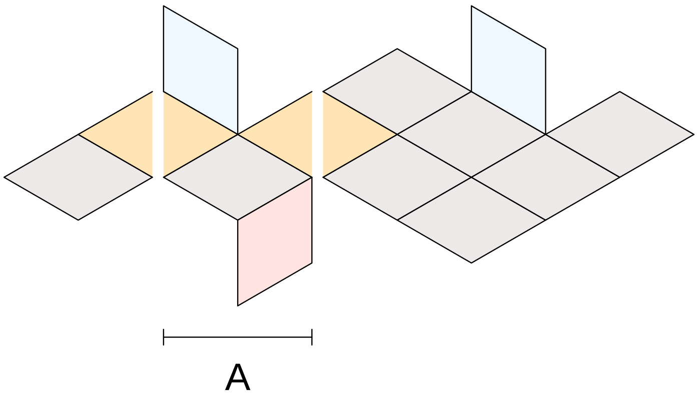


**Figure A17.** Construction 17 gives tilings with $\tau = 2\rho - 1$ for odd $\rho \geq 5$. Segment A is repeated $a$ times ($a \geq 0$), giving $\tau = 9 + 4a$ and $\rho = 5 + 2a$.

## Internal Extension 18

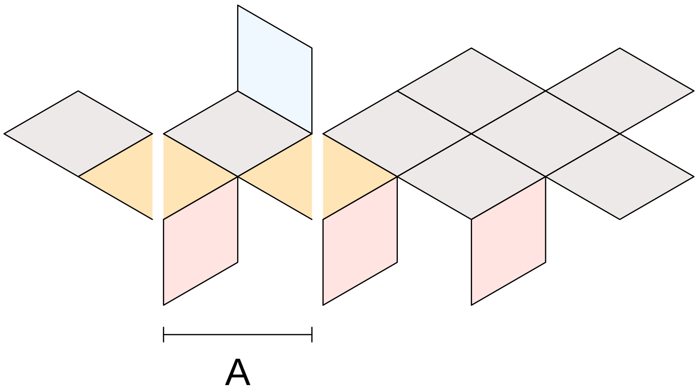


**Figure A18.** Construction 18 gives tilings with $\tau = 2\rho$ for odd $\rho \geq 5$. Segment A is repeated $a$ times ($a \geq 0$), giving $\tau = 10 + 4a$ and $\rho = 5 + 2a$.

## Internal Extension 19

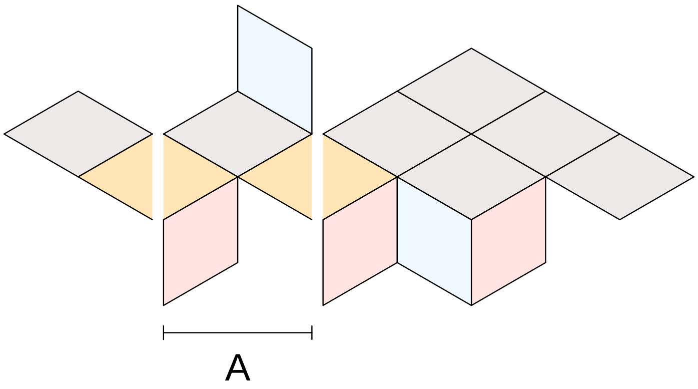


**Figure A19.** Construction 19 gives tilings with $\tau = 2\rho - 2$ for even $\rho \geq 6$. Segment A is repeated $a$ times ($a \geq 0$), giving $\tau = 10 + 4a$ and $\rho = 6 + 2a$.

## Internal Extension 20

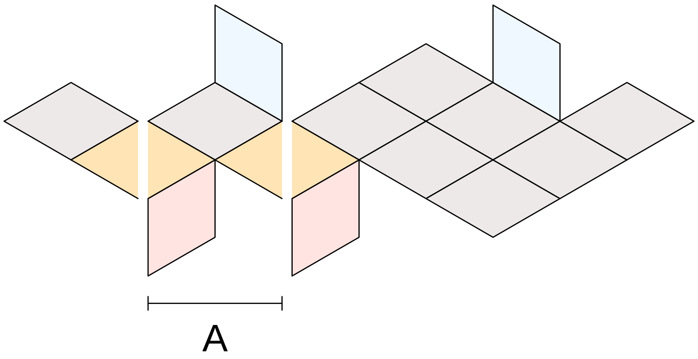


**Figure A20.** Construction 20 gives tilings with $\tau = 2\rho - 1$ for even $\rho \geq 6$. Segment A is repeated $a$ times ($a \geq 0$), giving $\tau = 11 + 4a$ and $\rho = 6 + 2a$.

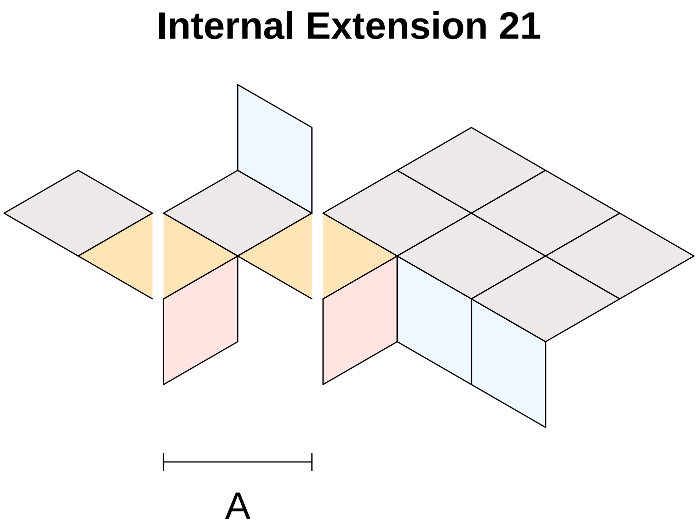


**Figure A21.** Construction 21 gives tilings with $\tau = 2\rho - 3$ for odd $\rho \geq 7$. Segment A is repeated $a$ times ($a \geq 0$), giving $\tau = 11 + 4a$ and $\rho = 7 + 2a$.

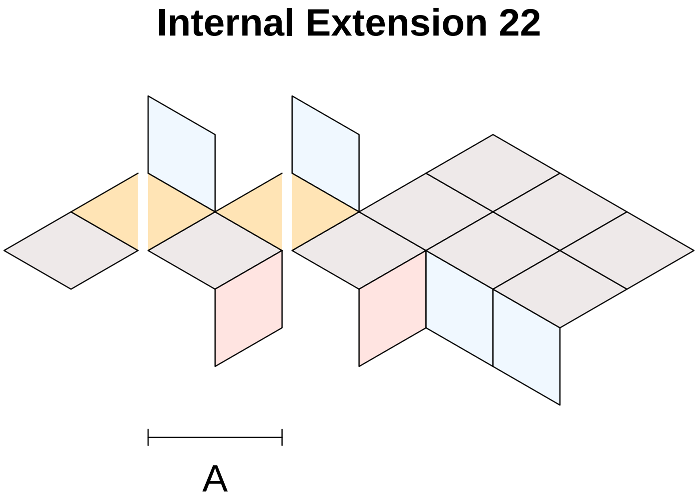


**Figure A22.** Construction 22 gives tilings with $\tau = 2\rho - 3$ for even $\rho \geq 8$. Segment A is repeated $a$ times ($a \geq 0$), giving $\tau = 13 + 4a$ and $\rho = 8 + 2a$.

## Internal Extension 23

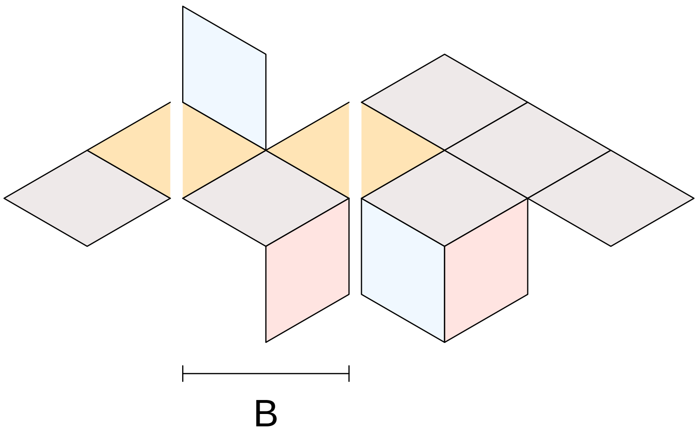


**Figure A23.** Construction 23 gives tilings with $\tau = 2\rho - 2$ for odd $\rho \geq 7$. Segment B is repeated $b$ times ($b \geq 1$), giving $\tau = 8 + 4b$ and $\rho = 5 + 2b$.

## Internal Extension 24

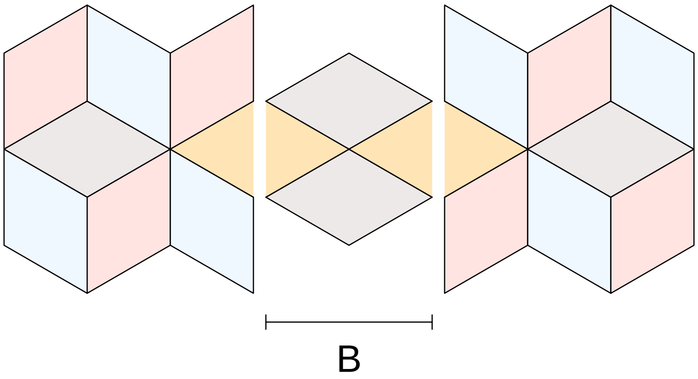


**Figure A24.** Construction 24 gives tilings with $\tau = 3\rho/2$ for even $\rho \geq 12$. Segment B is repeated $b$ times ($b \geq 1$), giving $\tau = 15 + 3b$ and $\rho = 10 + 2b$.

# Internal Extension 25

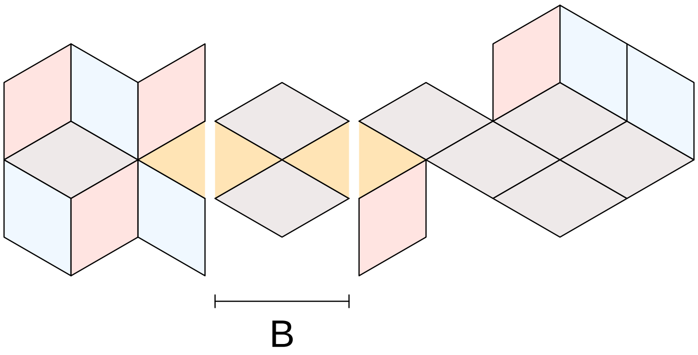


**Figure A25.** Construction 25 gives tilings with $\tau = (3\rho + 1)/2$ for odd $\rho \geq 13$. Segment B is repeated $b$ times ($b \geq 1$), giving $\tau = 17 + 3b$ and $\rho = 11 + 2b$.

# External Extension 1

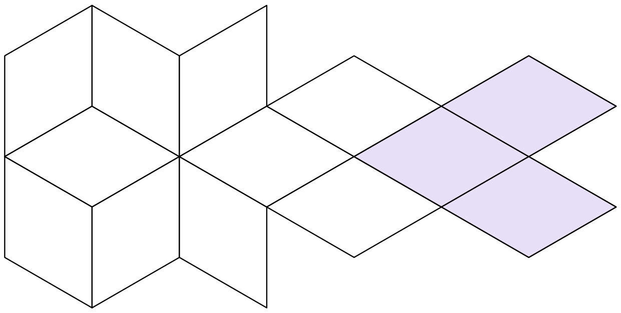

**Figure A26.** The tiling dap10.6o (white tiles) may be extended on the right by adding the 3-tile pattern shown in purple as many times as desired, increasing the number of runs by two each time.

## External Extension 2

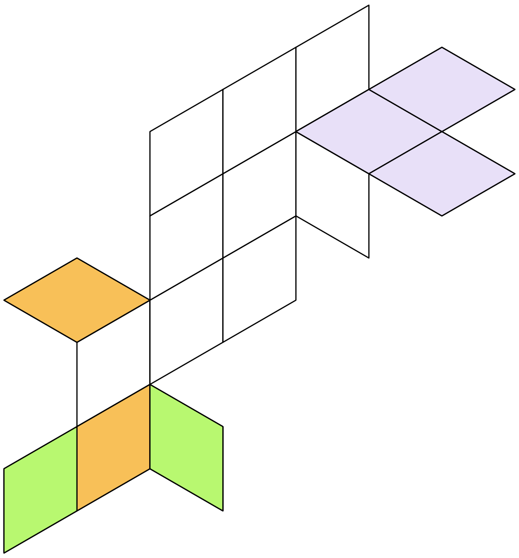

**Figure A27.** The tiling dap9.5b (white tiles) may be extended on the right by adding the 3-tile pattern shown in purple as many times as desired, increasing the number of runs by two each time. It may also be extended on the left, by first attaching the two tiles shown in orange to the leftmost tile and then attaching the two green tiles to the upper orange tile, again increasing the number of runs by two. This may also be repeated as many times as desired and the addition of the green tiles may be omitted on the last repetition.

## External Extension 3

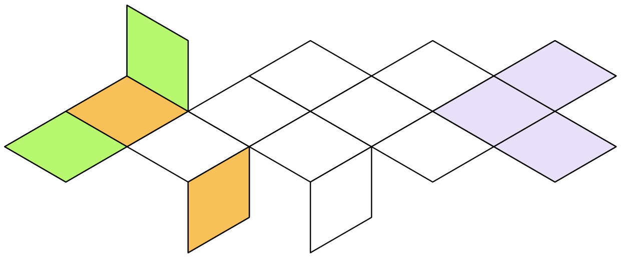

**Figure A28.** The tiling dap8.4b (white tiles) may be extended on the right by adding the 3-tile pattern shown in purple as many times as desired, increasing the number of runs by two each time. It may also be extended on the left, by first attaching the two tiles shown in orange to the leftmost tile and then attaching the two green tiles to the upper orange tile, again increasing the number of runs by two. This may also be repeated as many times as desired and the addition of the green tiles may be omitted on the last repetition.
