# Supplementary material for: Professor Preece's tredoku tilings
Source: arXiv:2511.12680 ancillary file (2025-11-16)
Supplement: Supplementary file 2 [file Appendix_B.pdf]

## APPENDIX B

This appendix shows all the tredoku tilings that appear in Donald's notes. The tilings are annotated as explained in Section 2.3 of the paper.

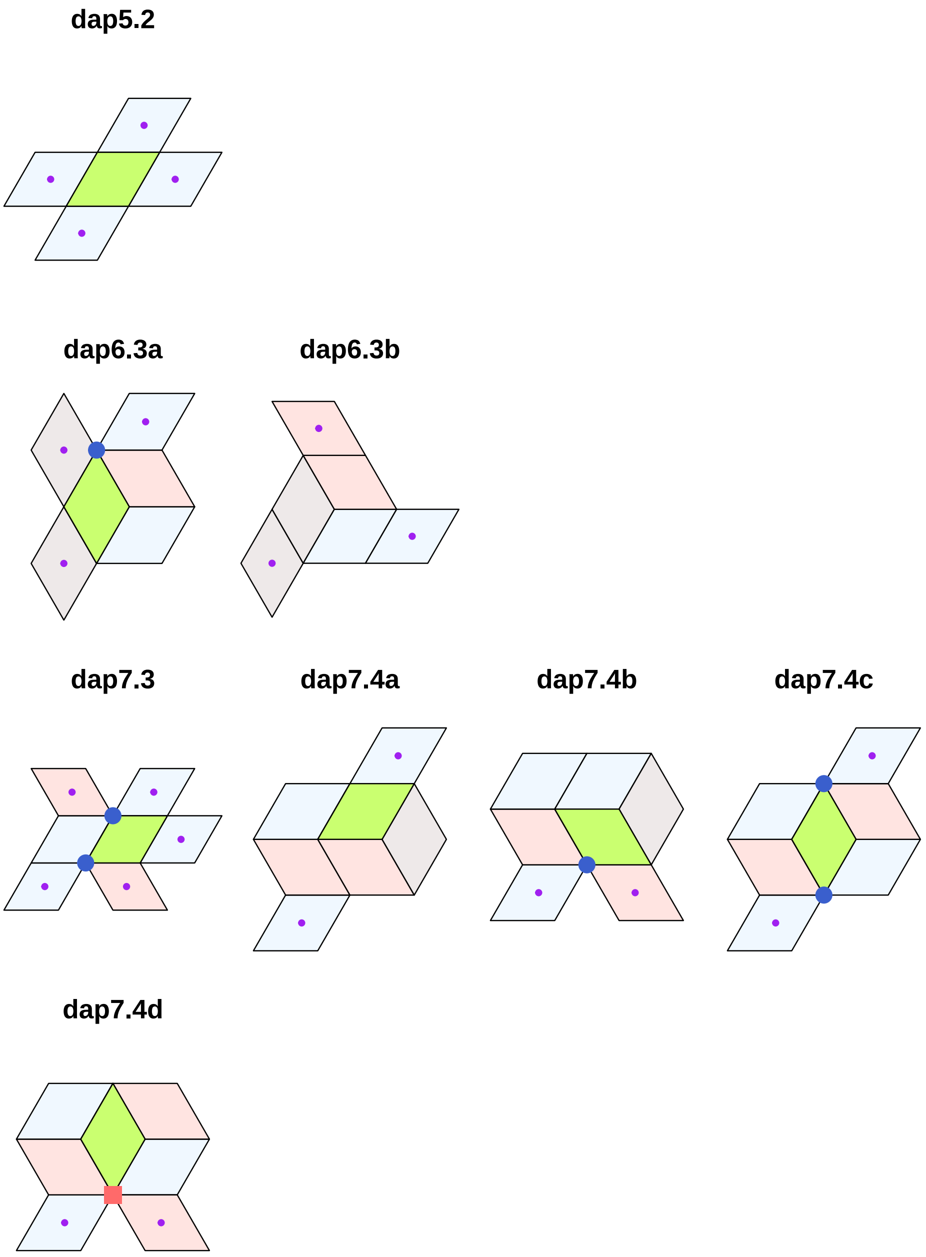


**Figure B1.** Tredoku tilings consisting of 5–7 tiles.

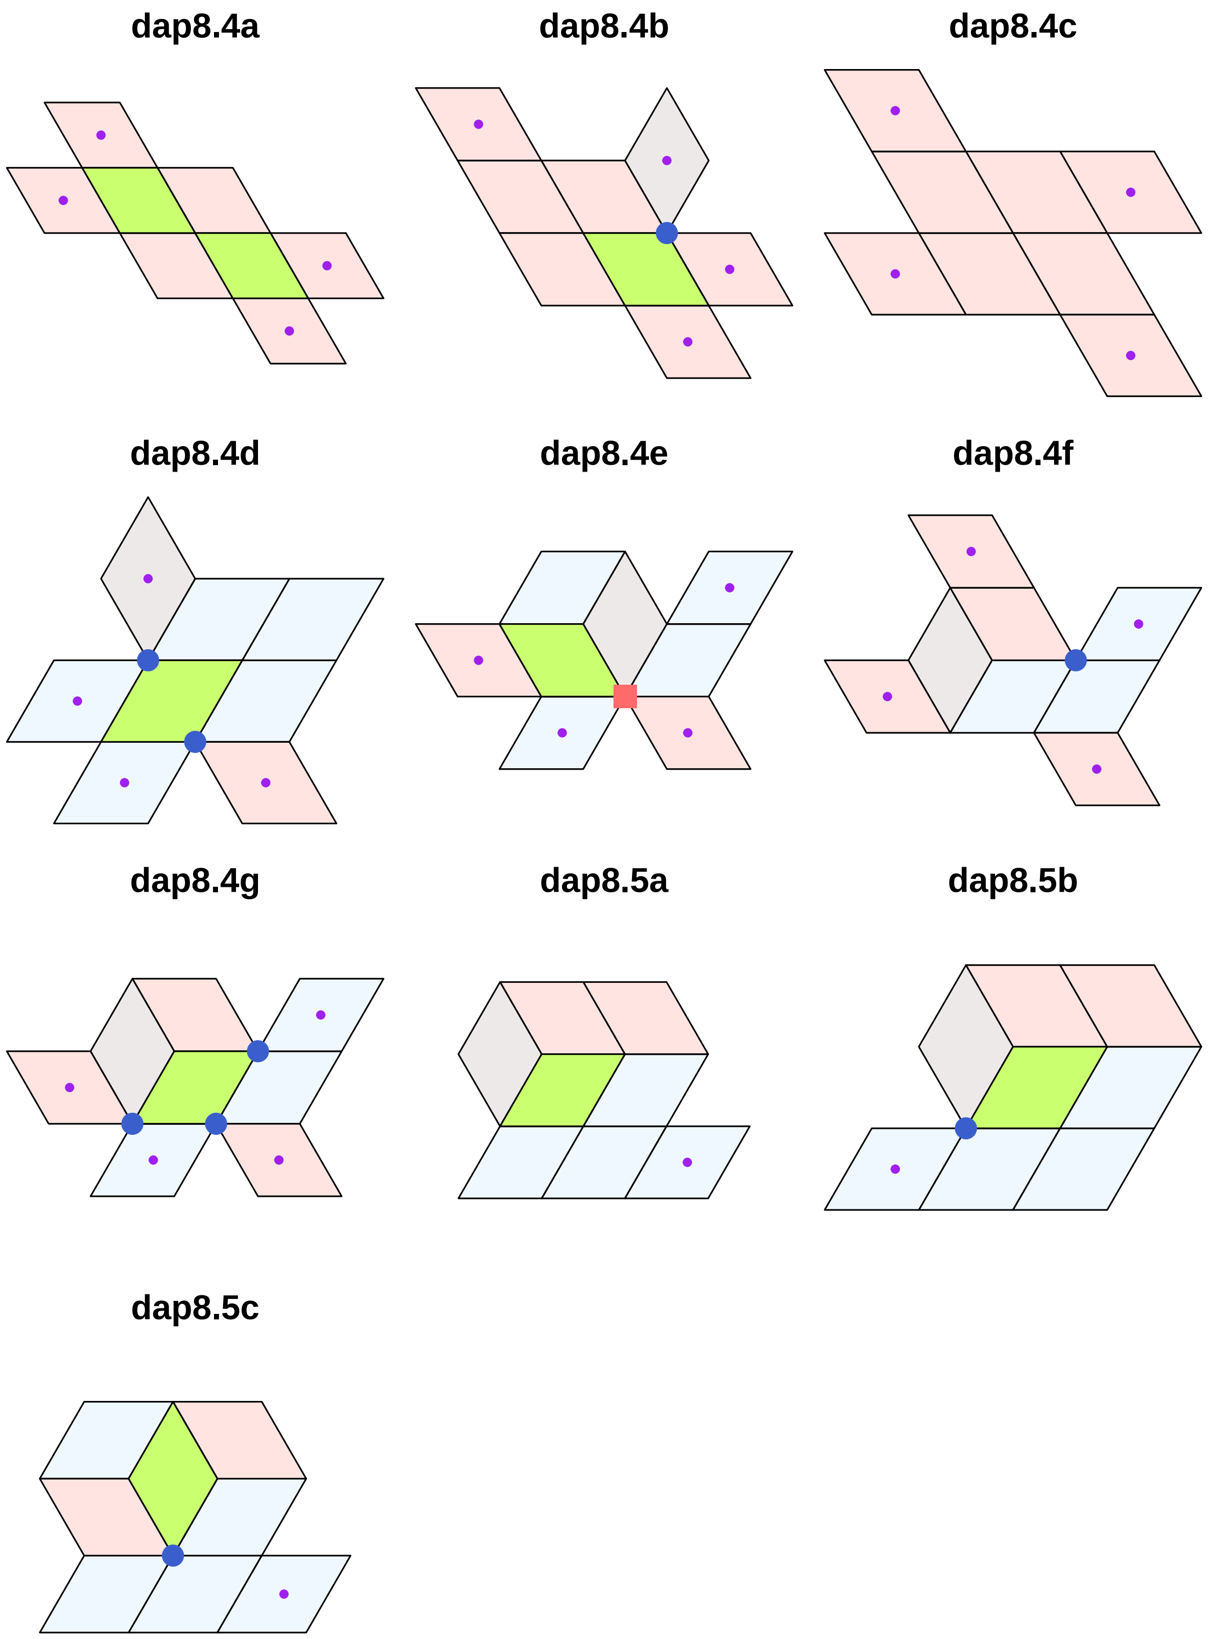


**Figure B2.** Tredoku tilings consisting of 8 tiles.

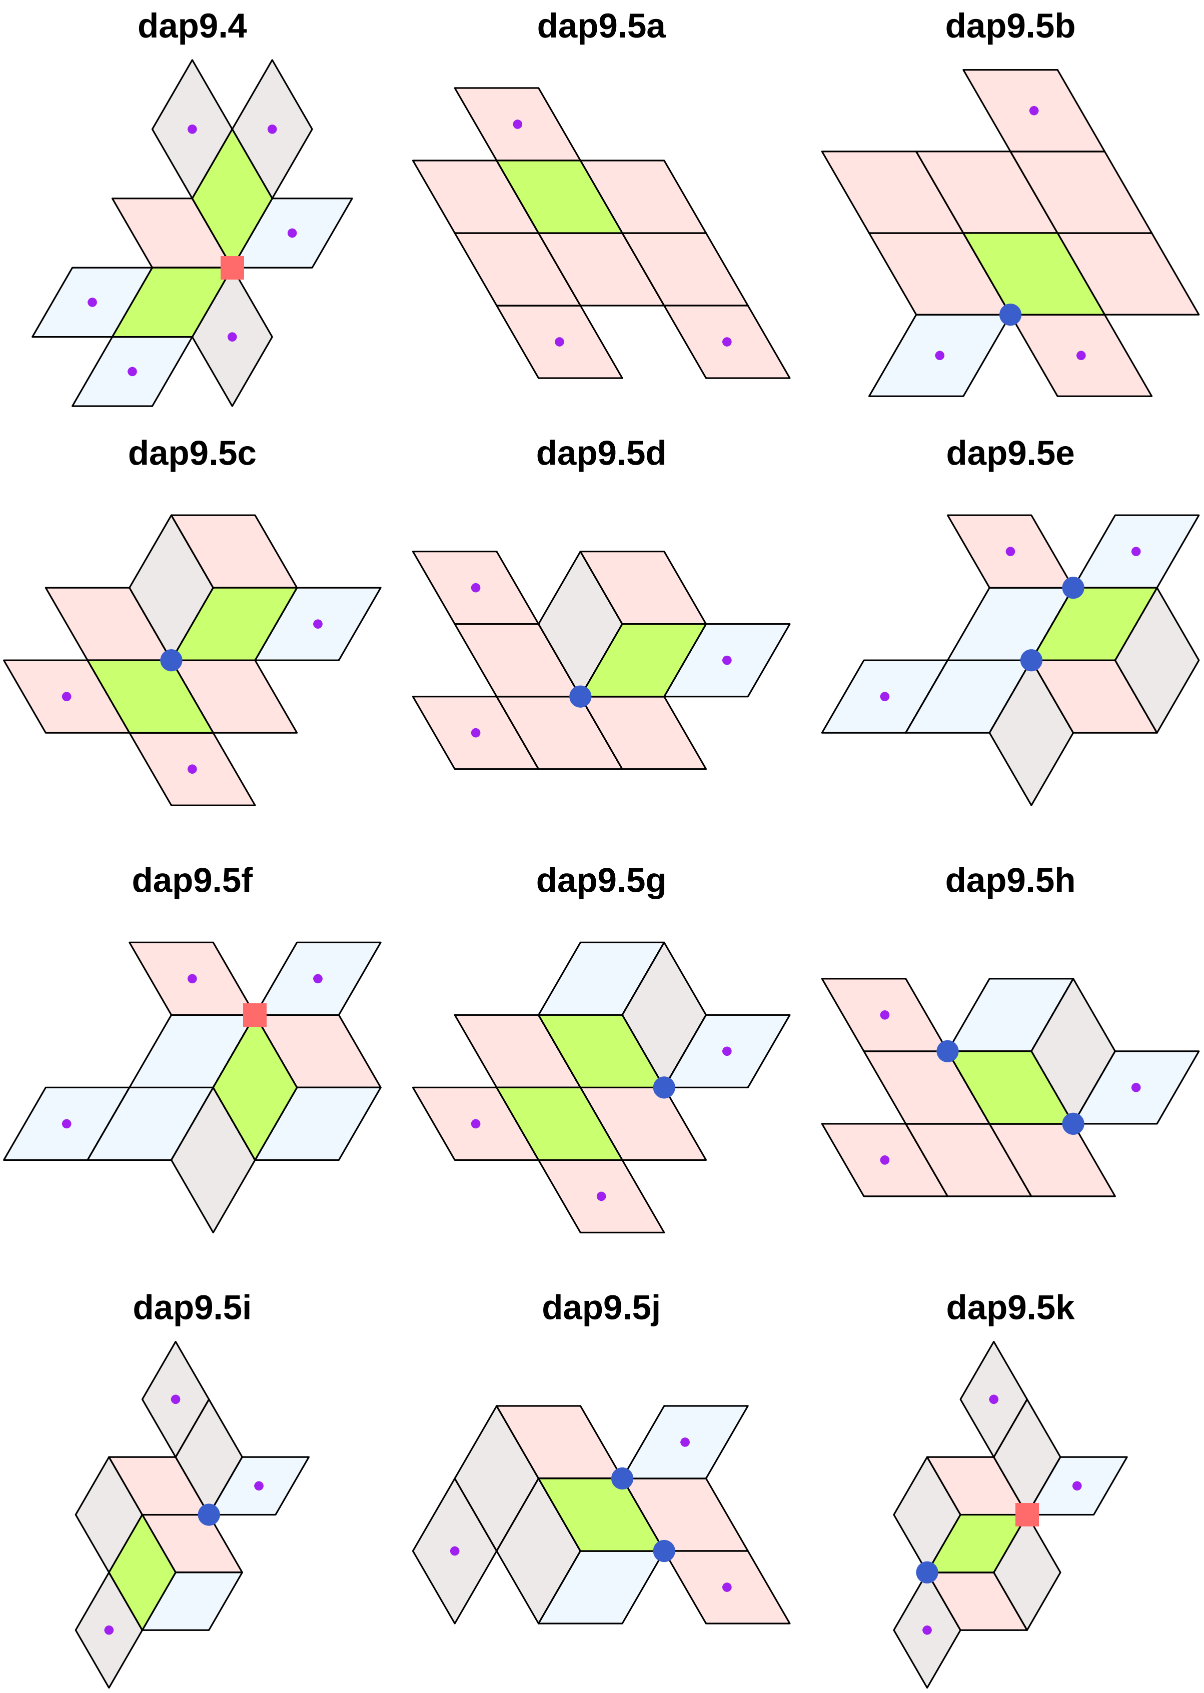


**Figure B3.** Tredoku tilings consisting of 9 tiles.

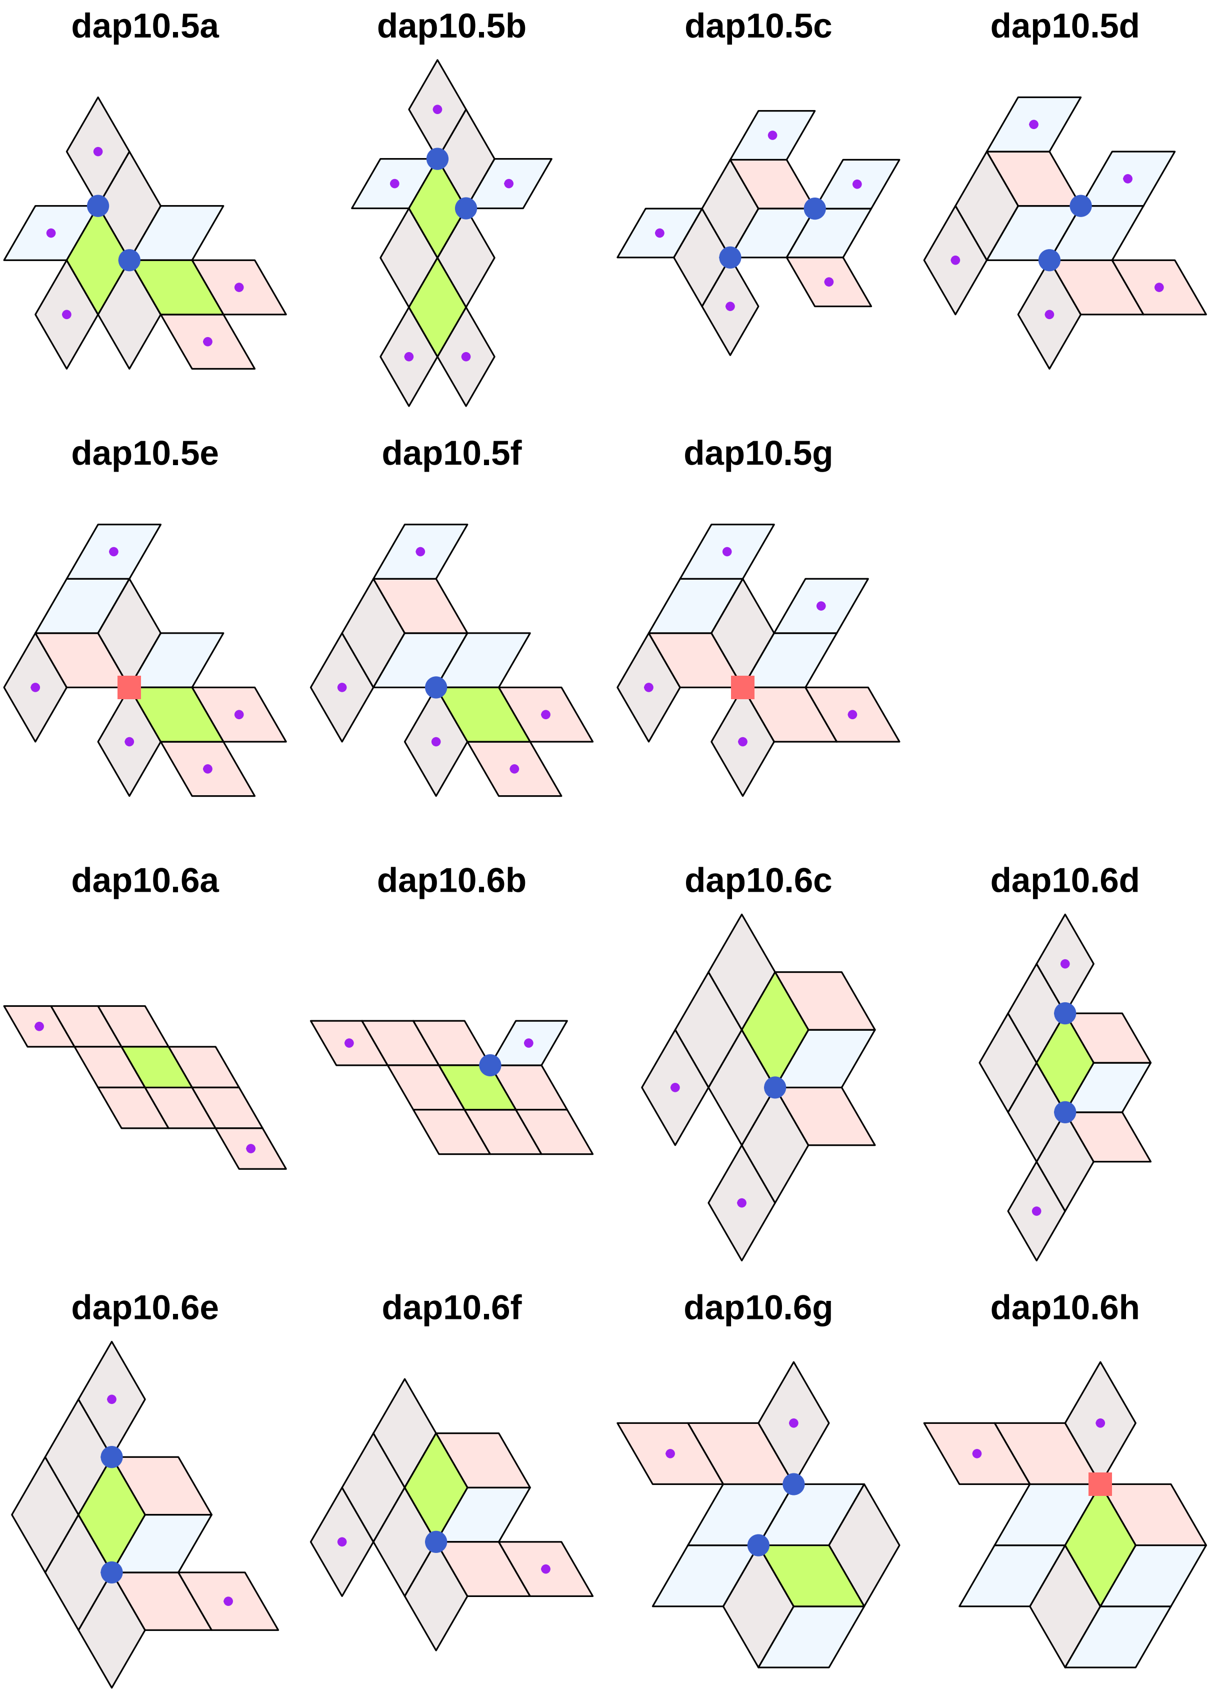


**Figure B4.** Tredoku tilings consisting of 10 tiles.

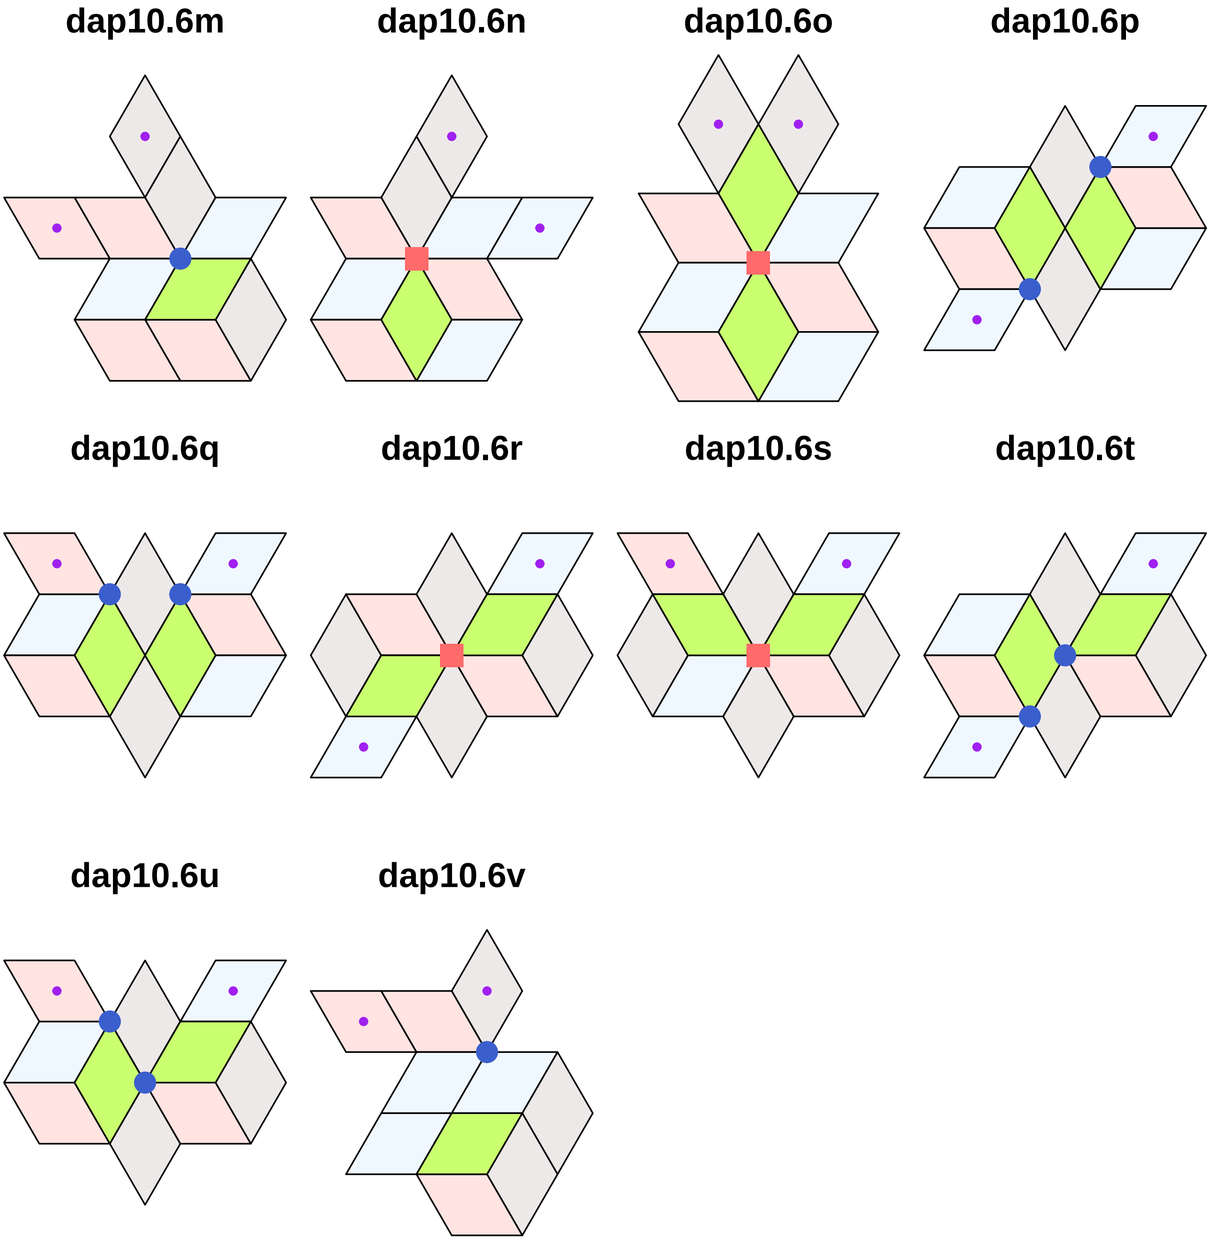


**Figure B5.** Tredoku tilings consisting of 10 tiles.

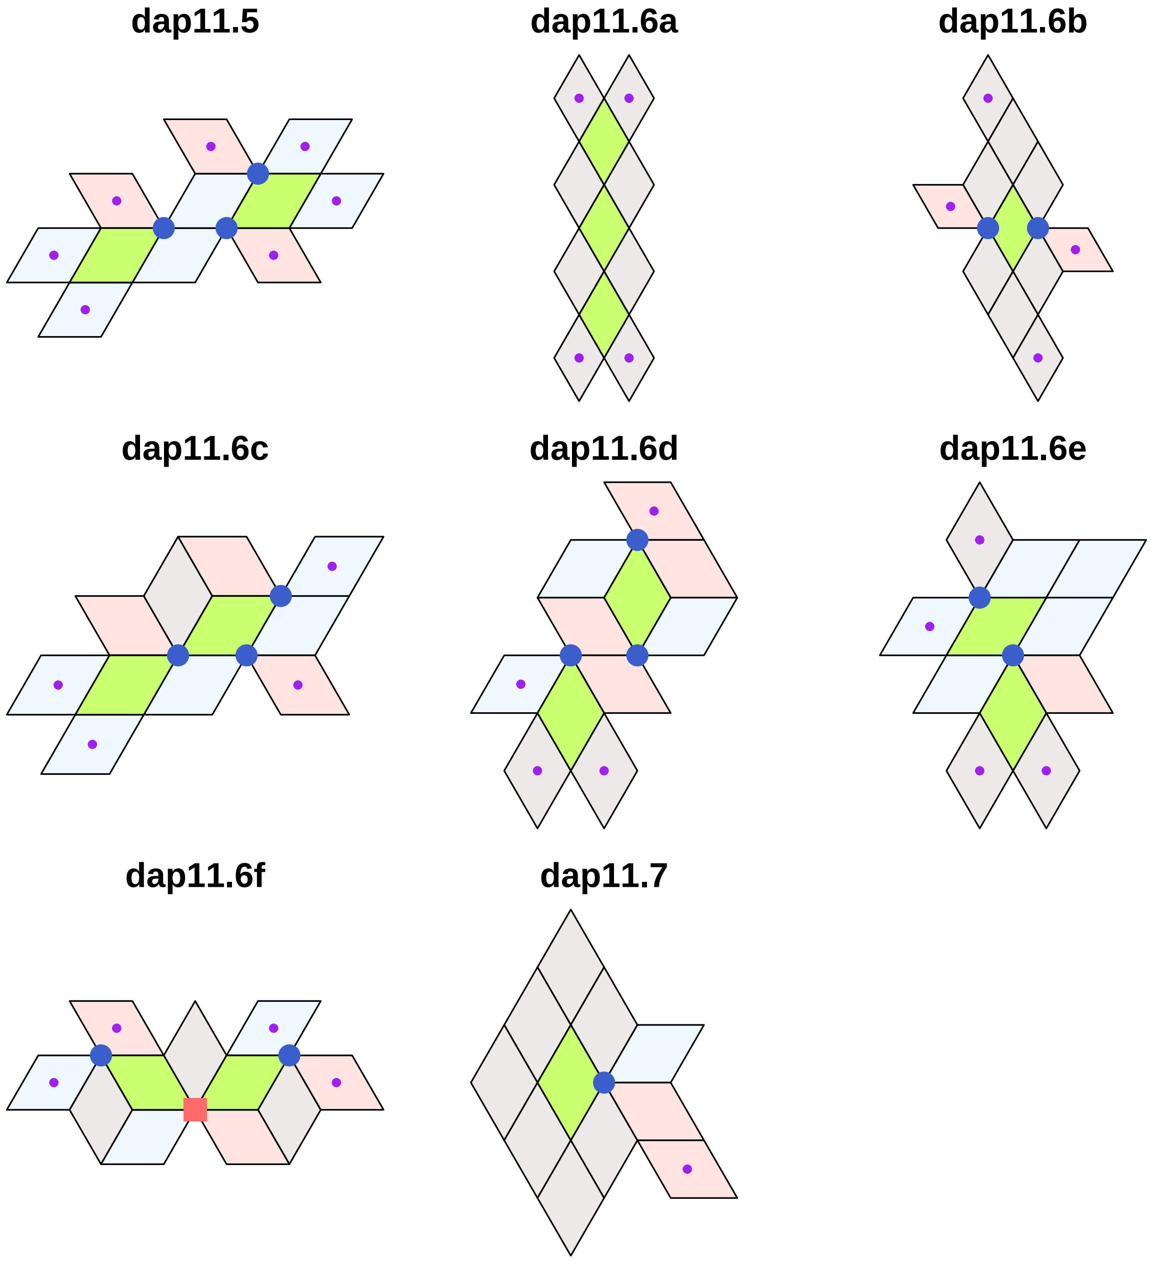


**Figure B6.** Tredoku tilings consisting of 11 tiles.

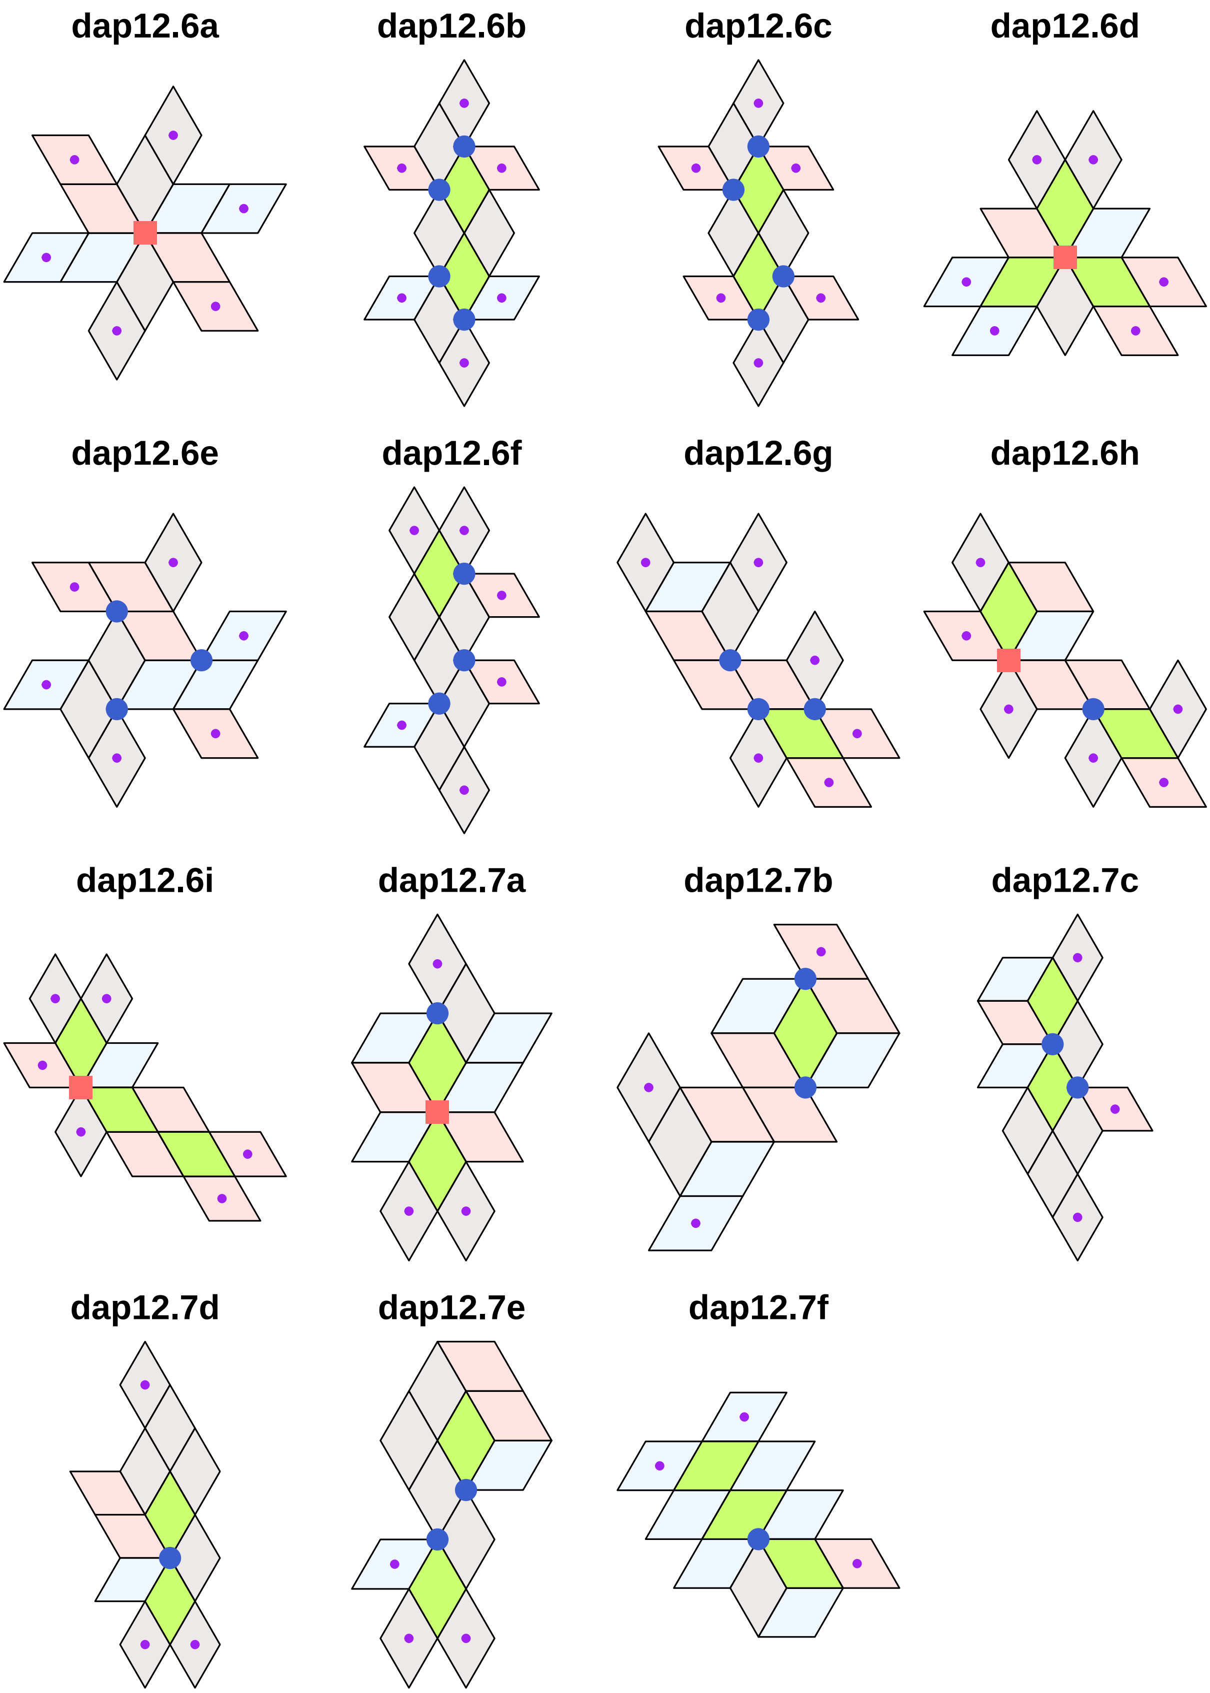


**Figure B7.** Tredoku tilings consisting of 12 tiles.

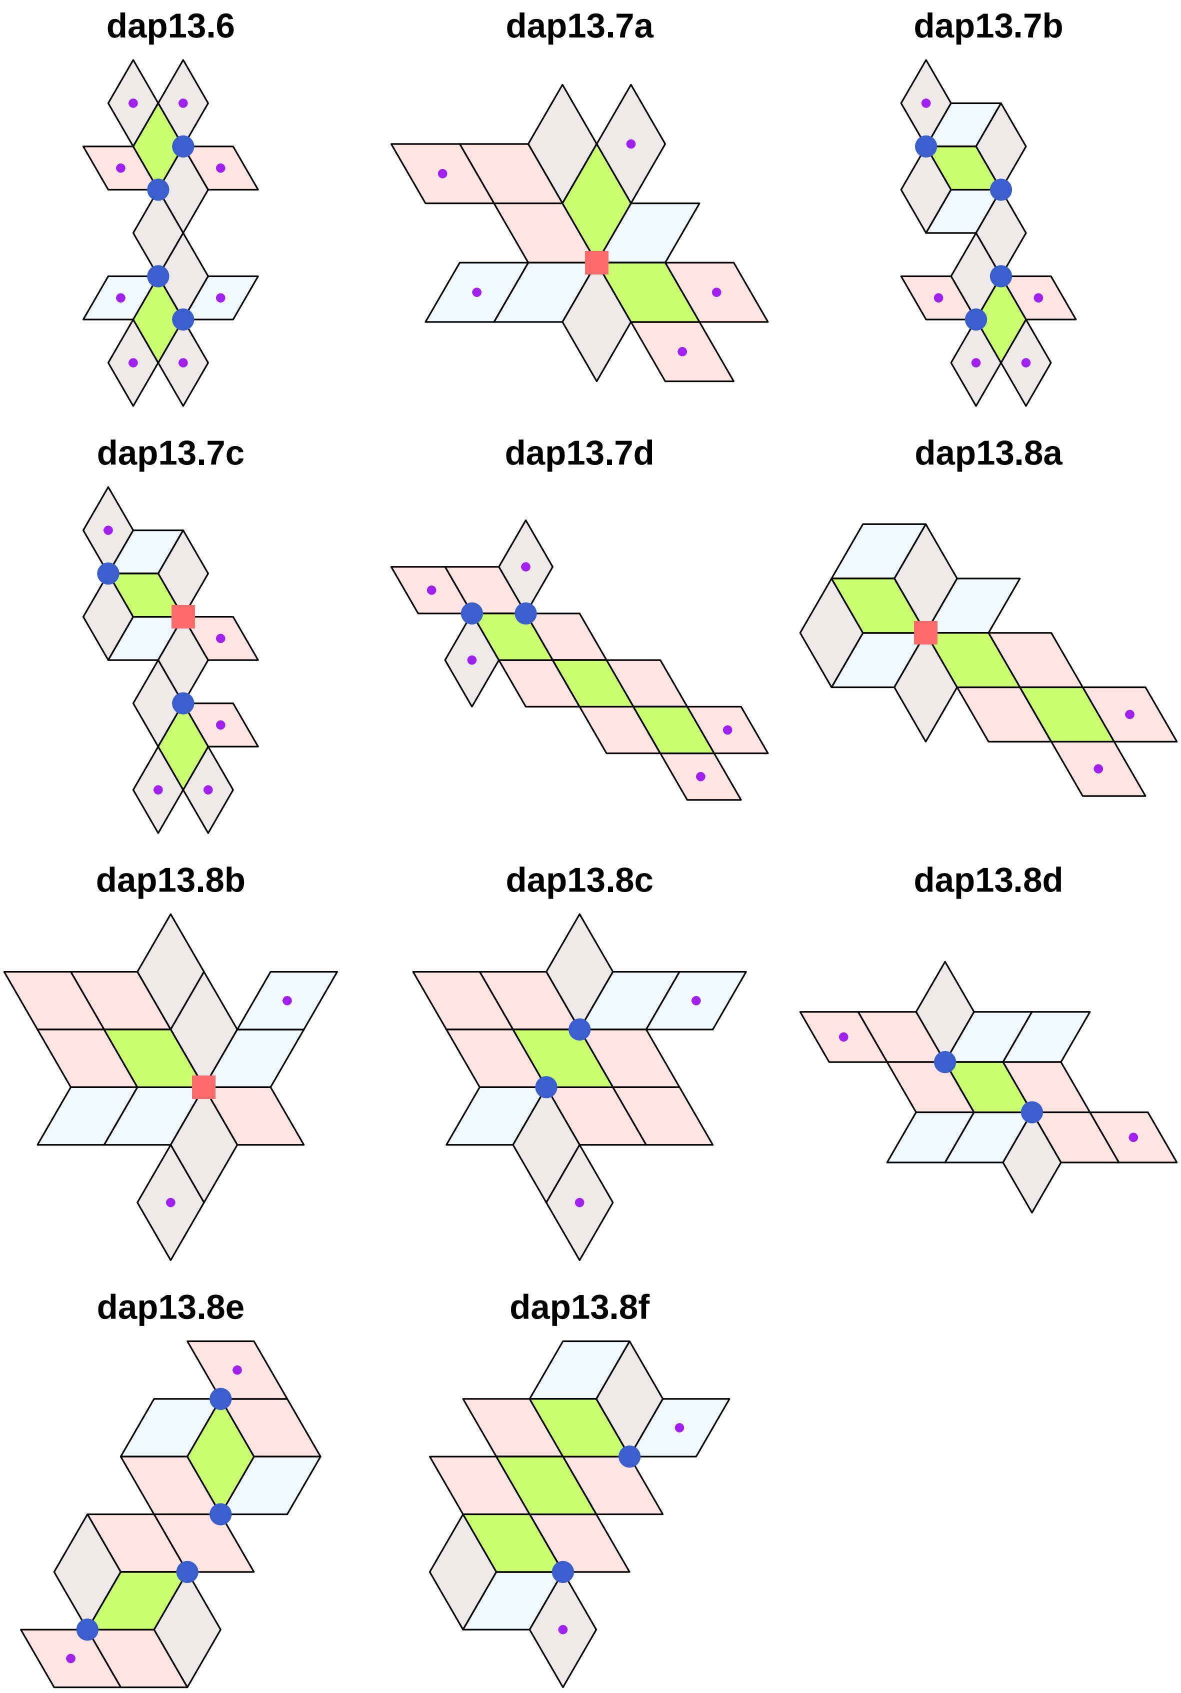


**Figure B8.** Tredoku tilings consisting of 13 tiles.

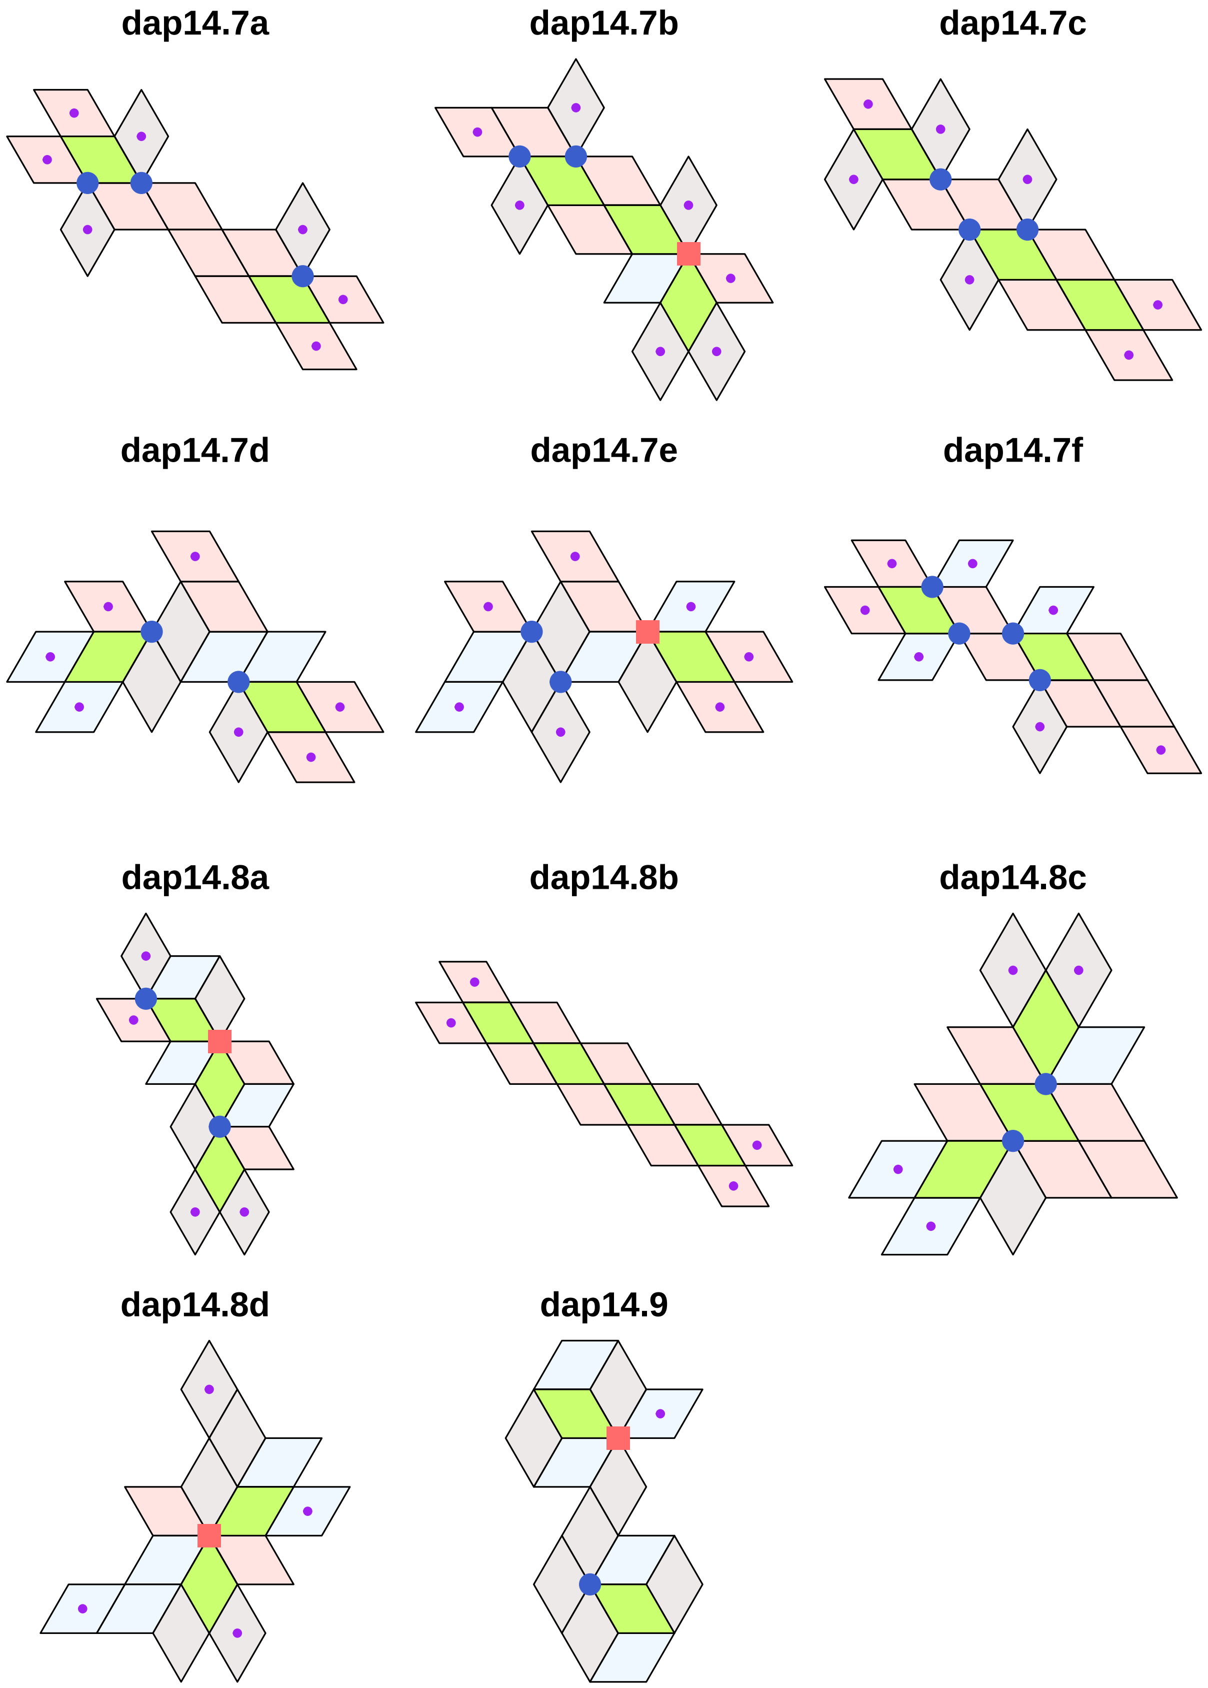


**Figure B9.** Tredoku tilings consisting of 14 tiles.

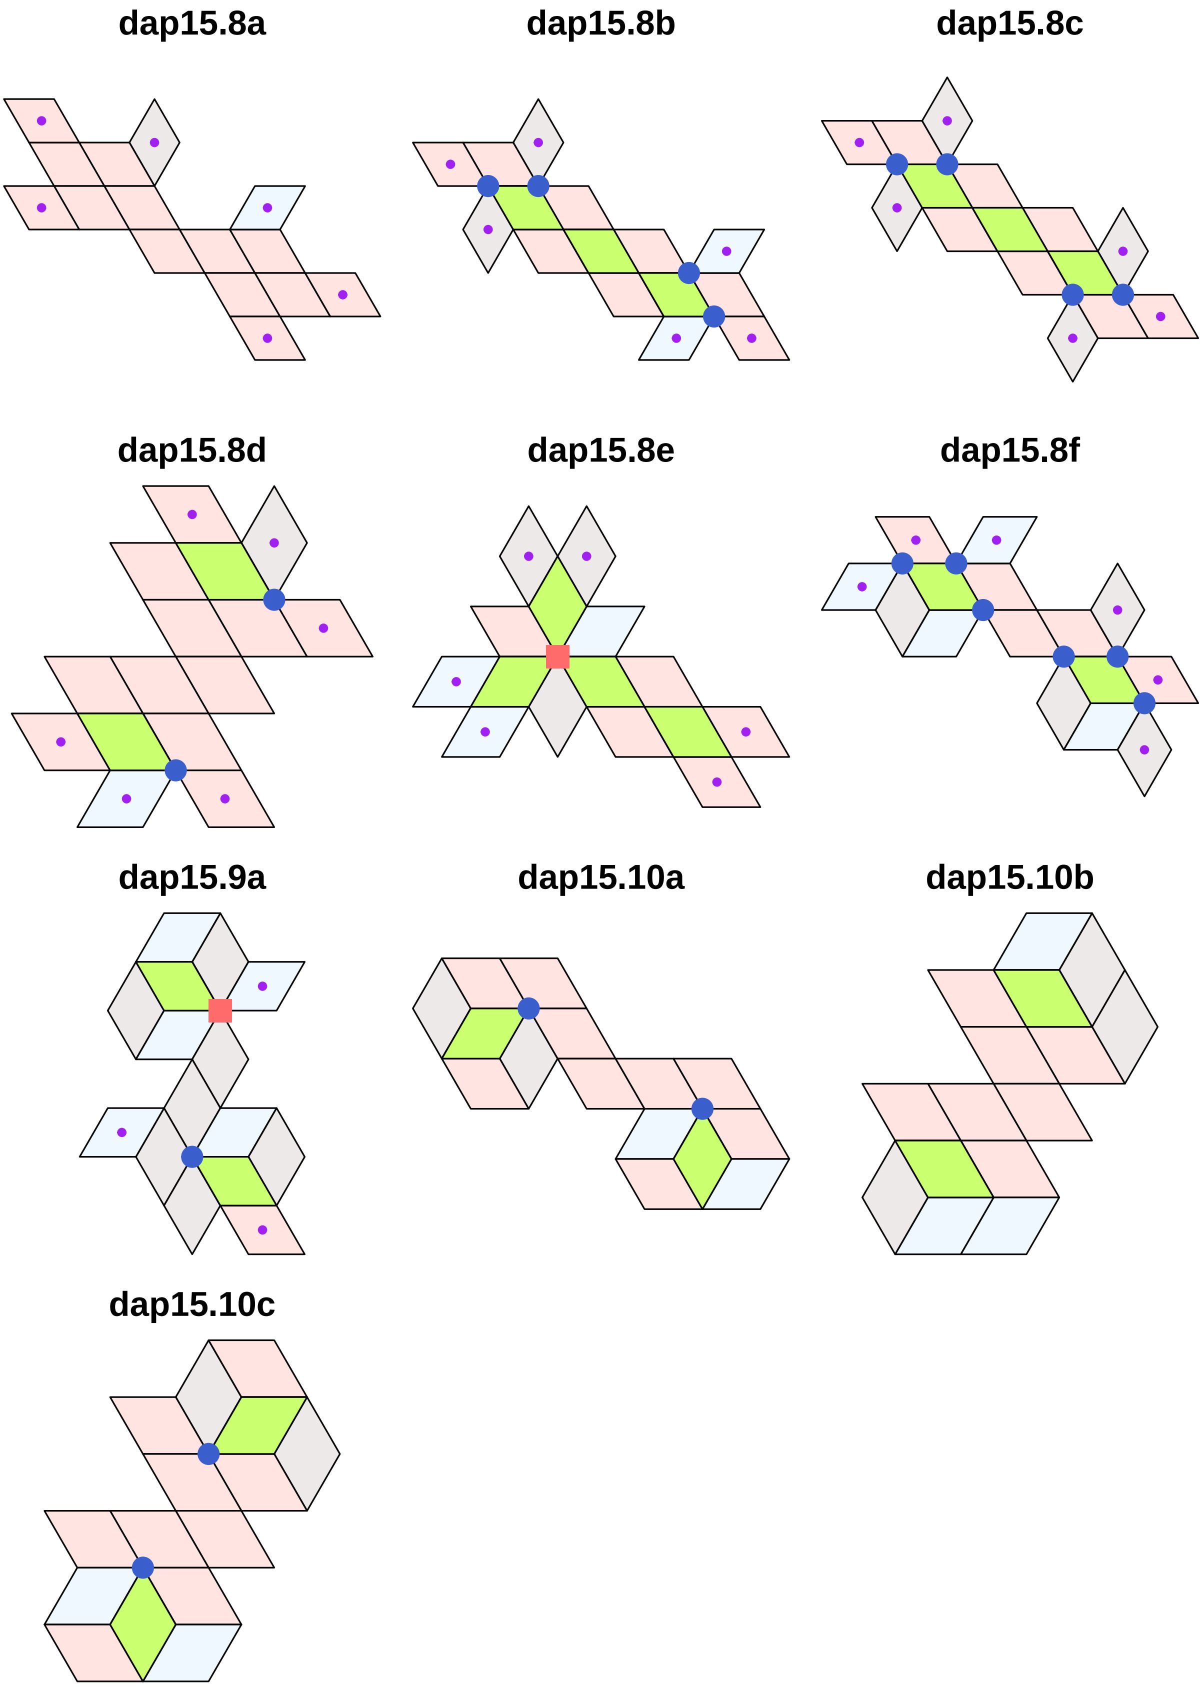


**Figure B10.** Tredoku tilings consisting of 15 tiles.

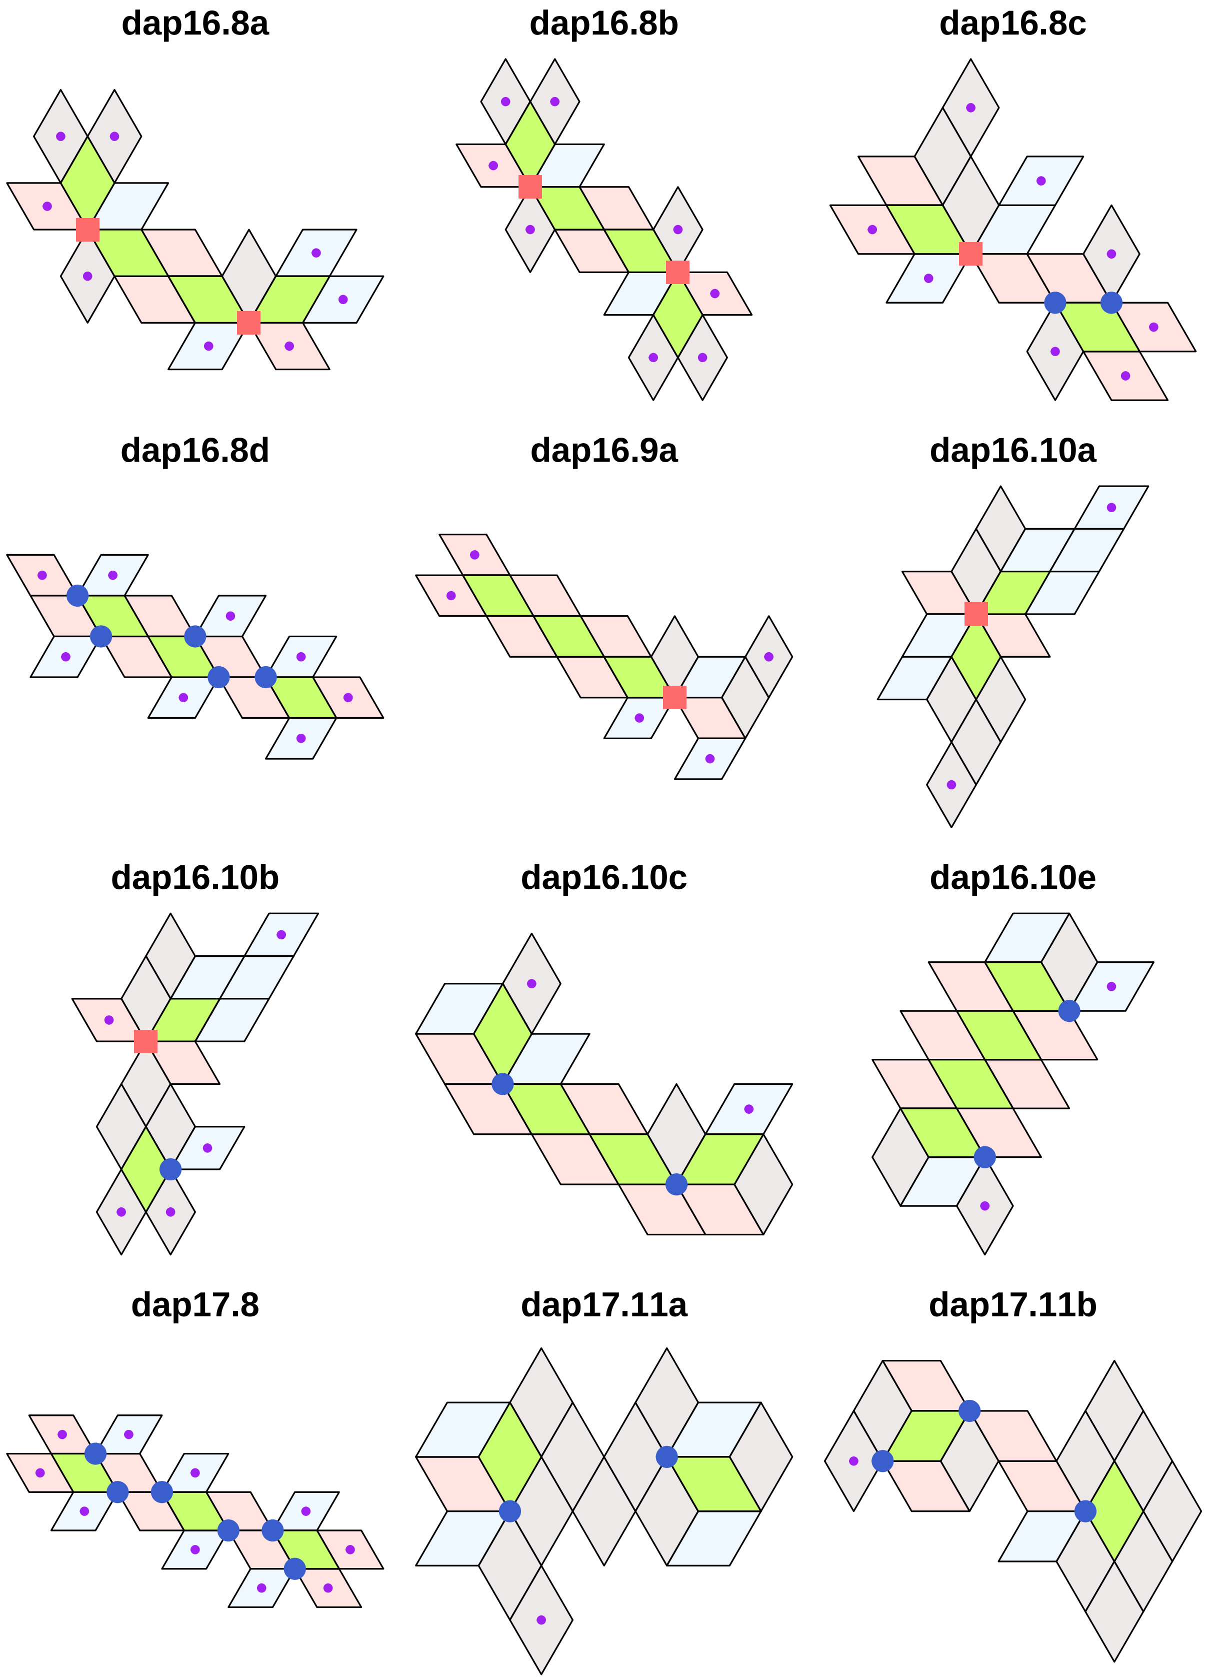


**Figure B11.** Tredoku tilings consisting of 16 or 17 tiles.

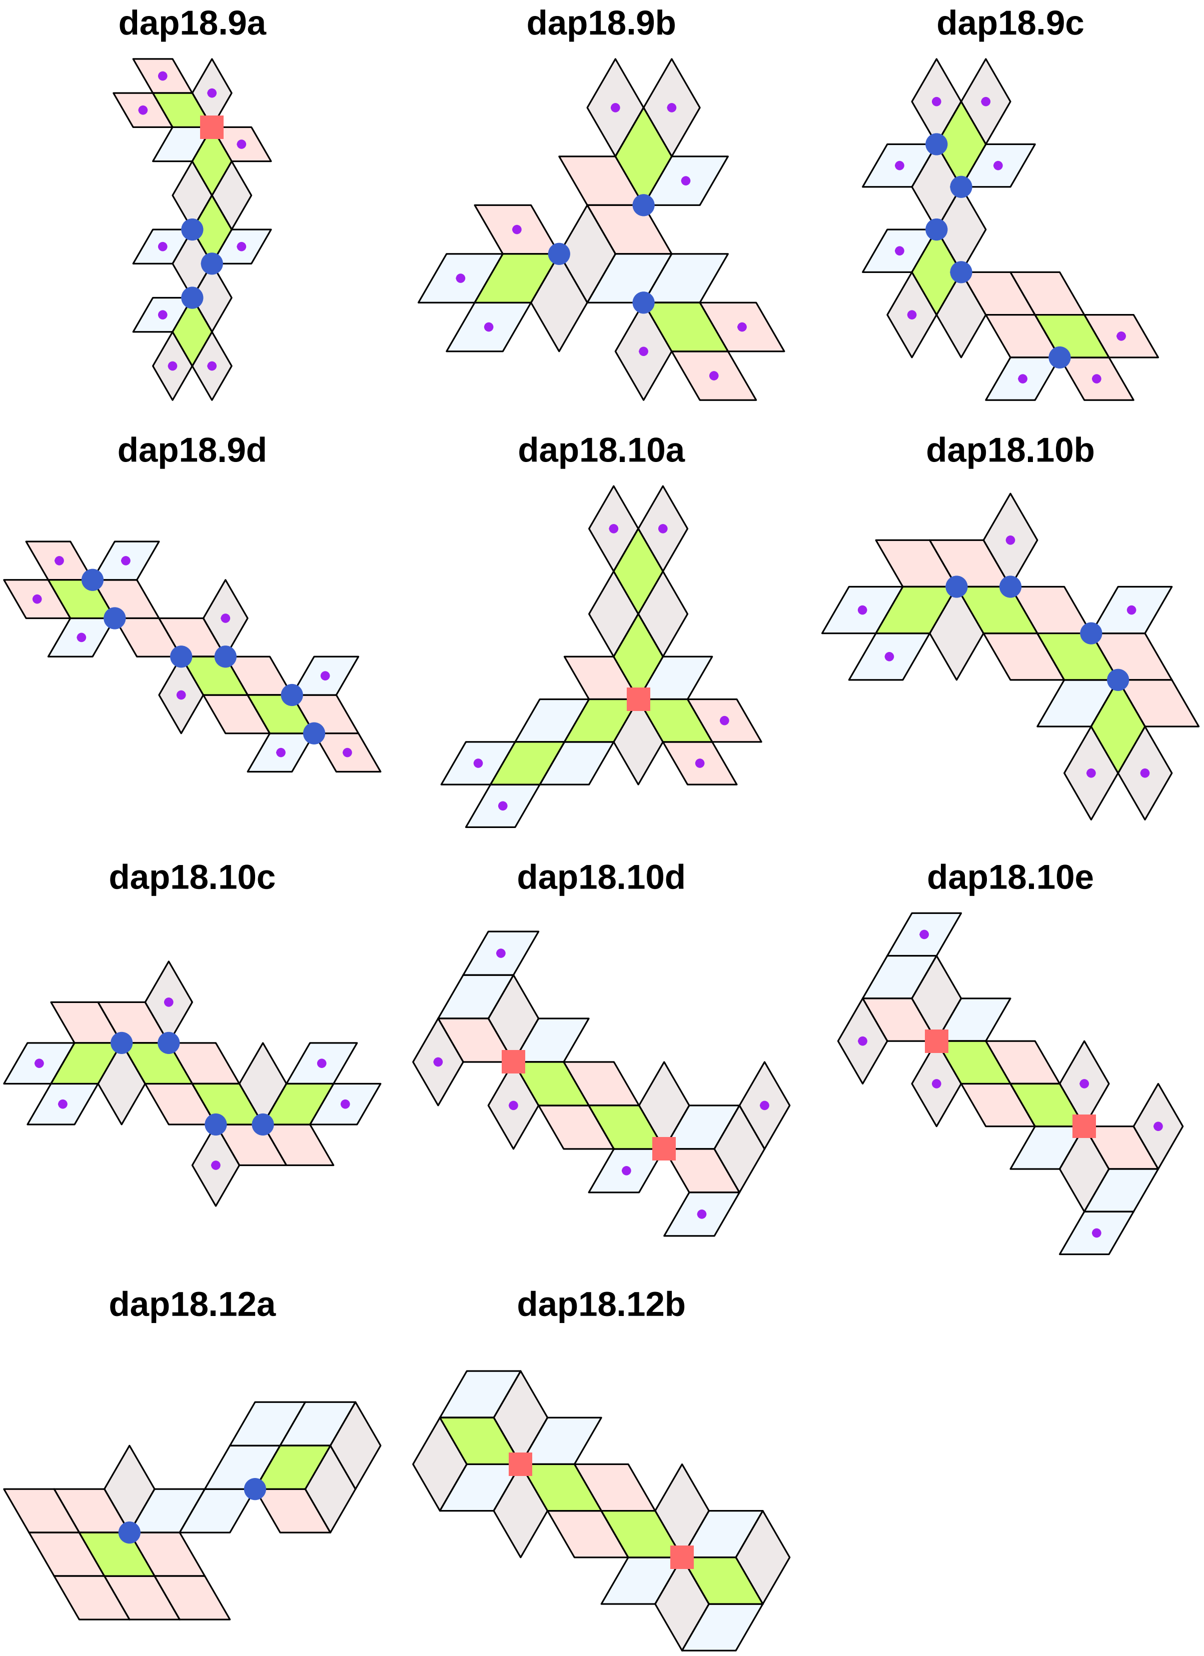


**Figure B12.** Tredoku tilings consisting of 18 tiles.

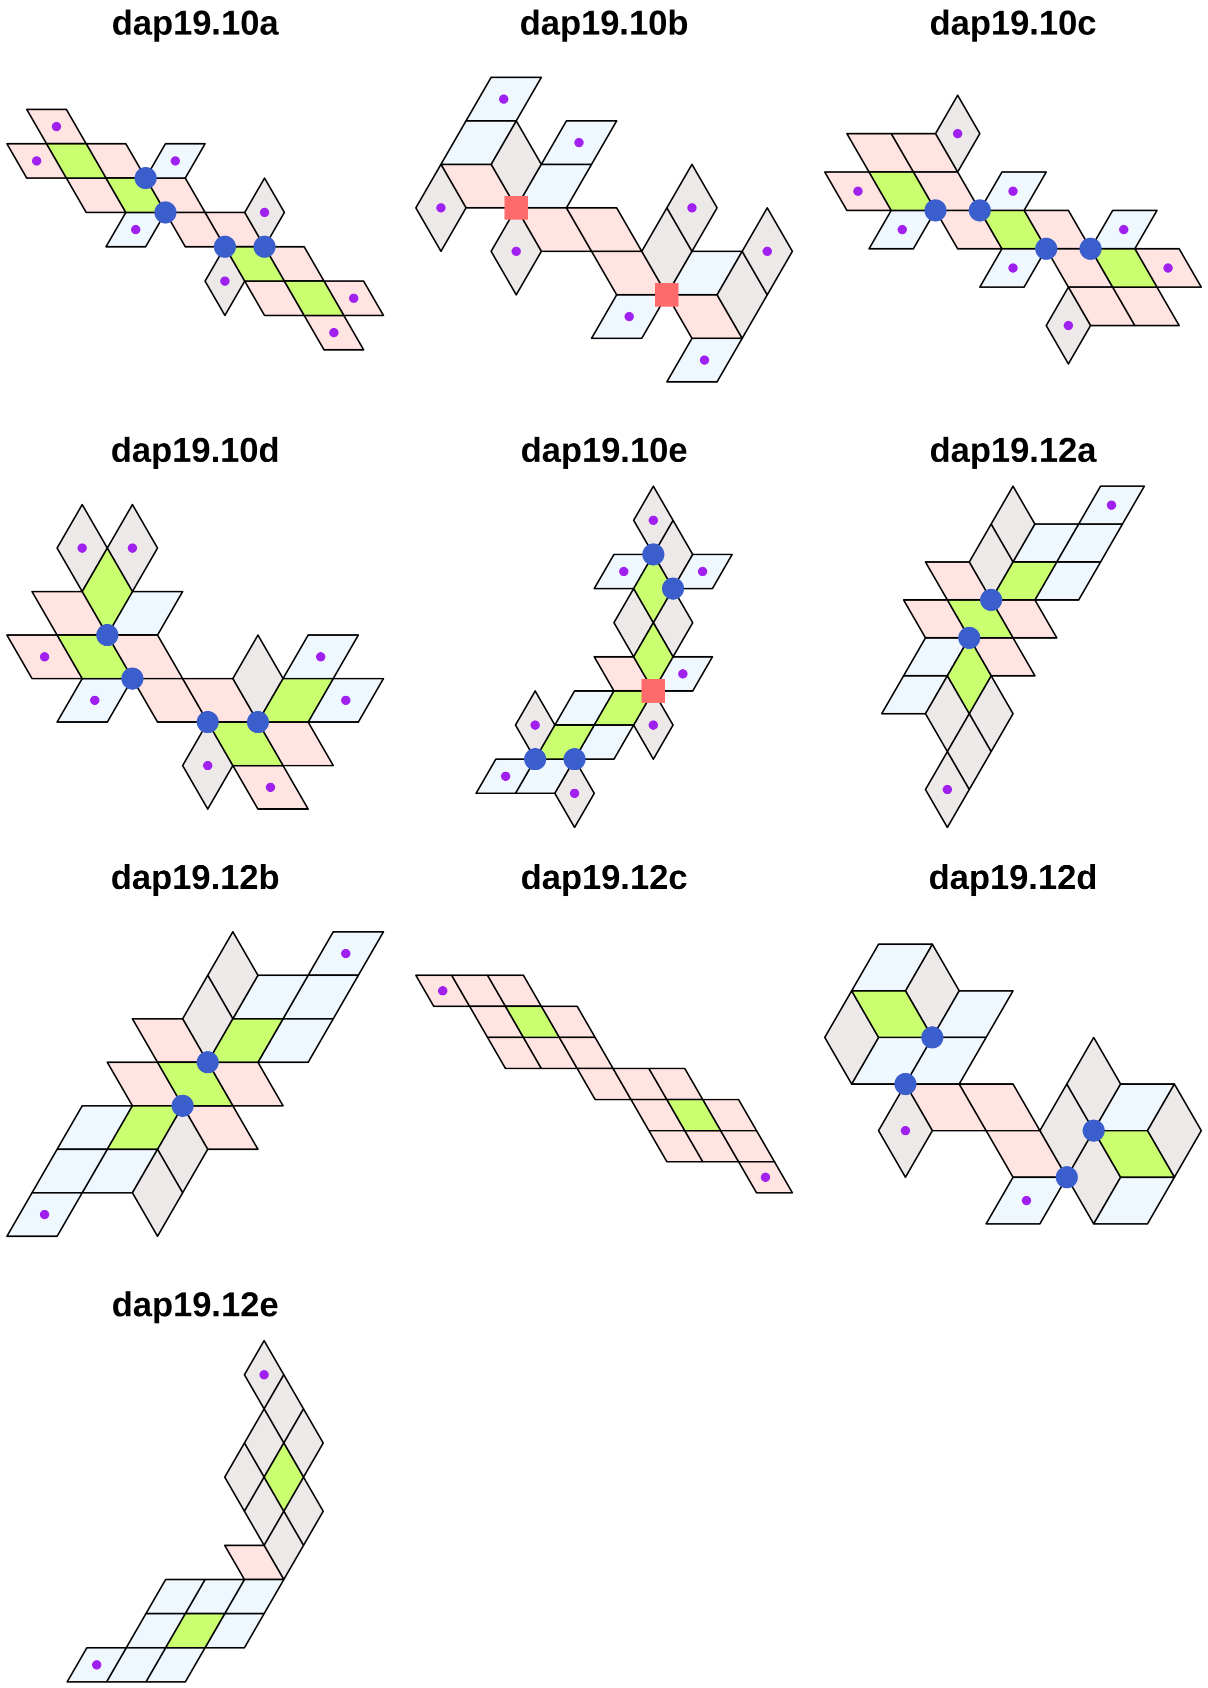


**Figure B13.** Tredoku tilings consisting of 19 tiles.

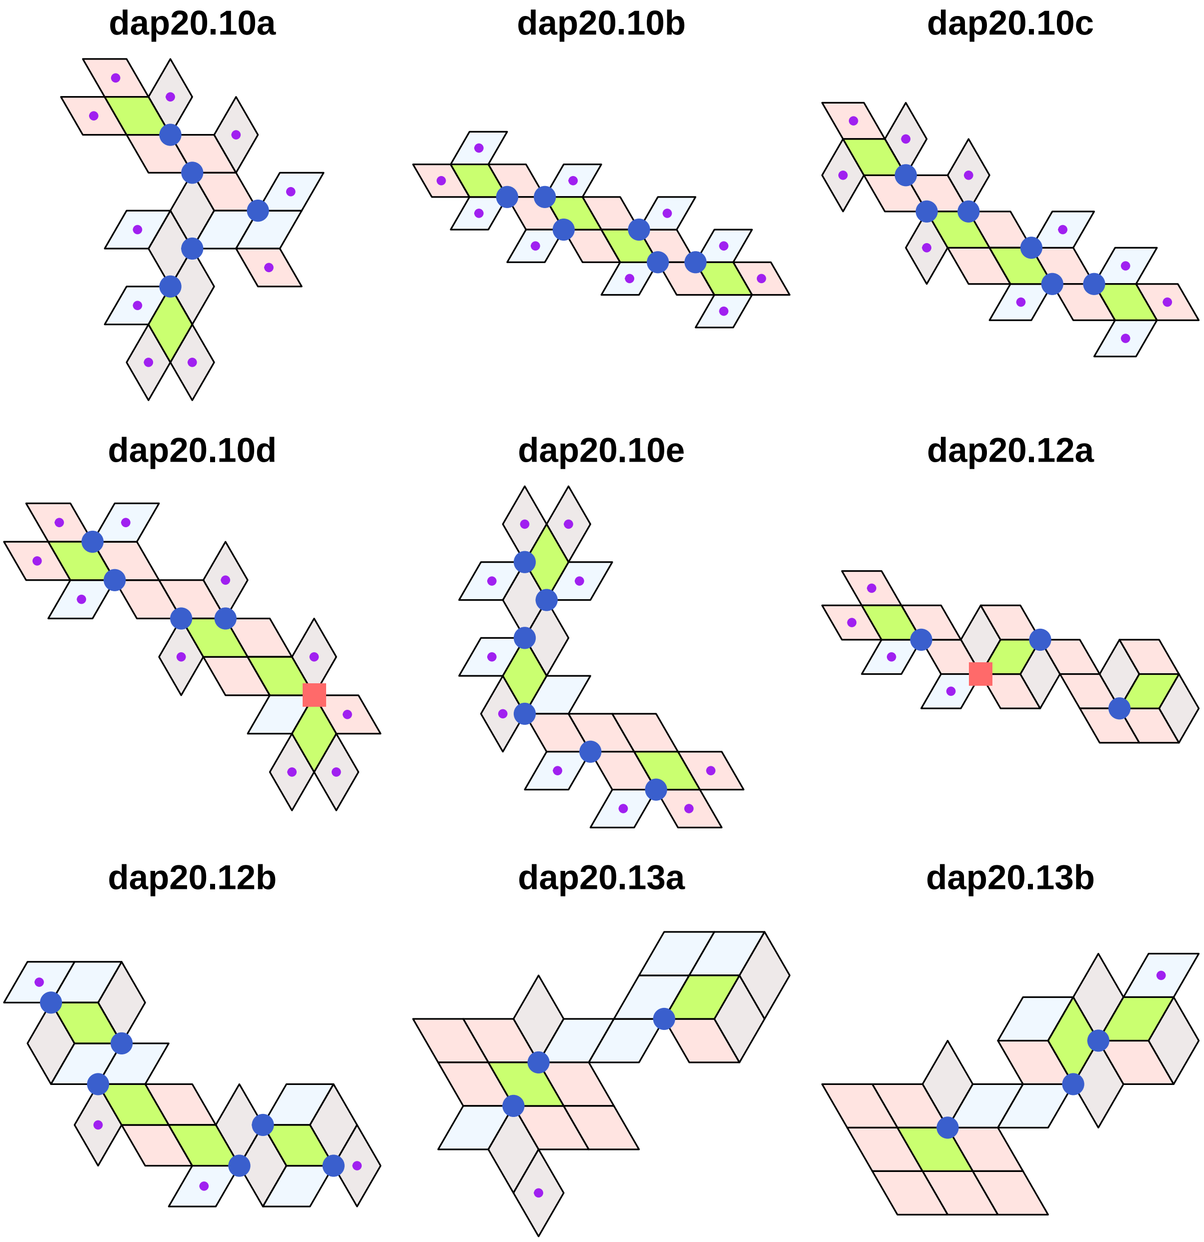


**Figure B14.** Tredoku tilings consisting of 20 tiles.

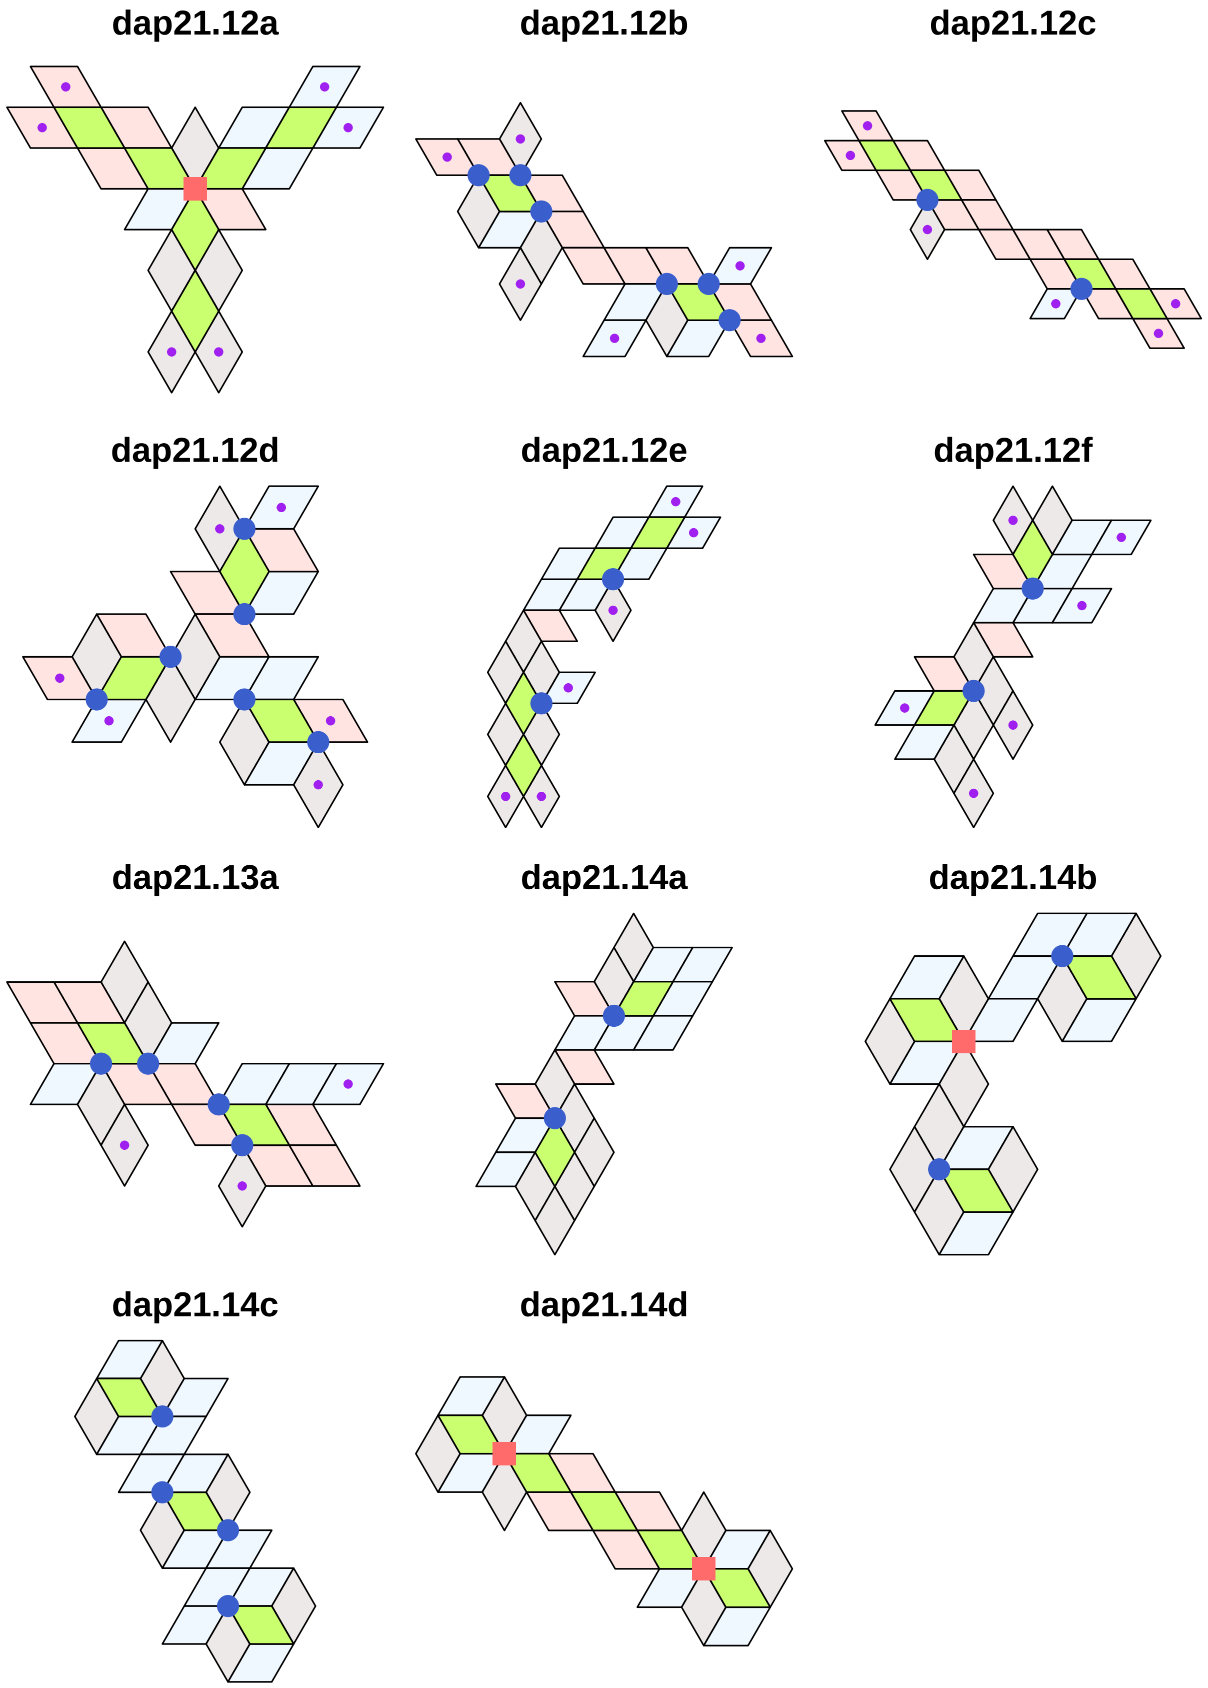


**Figure B15.** Tredoku tilings consisting of 21 tiles.

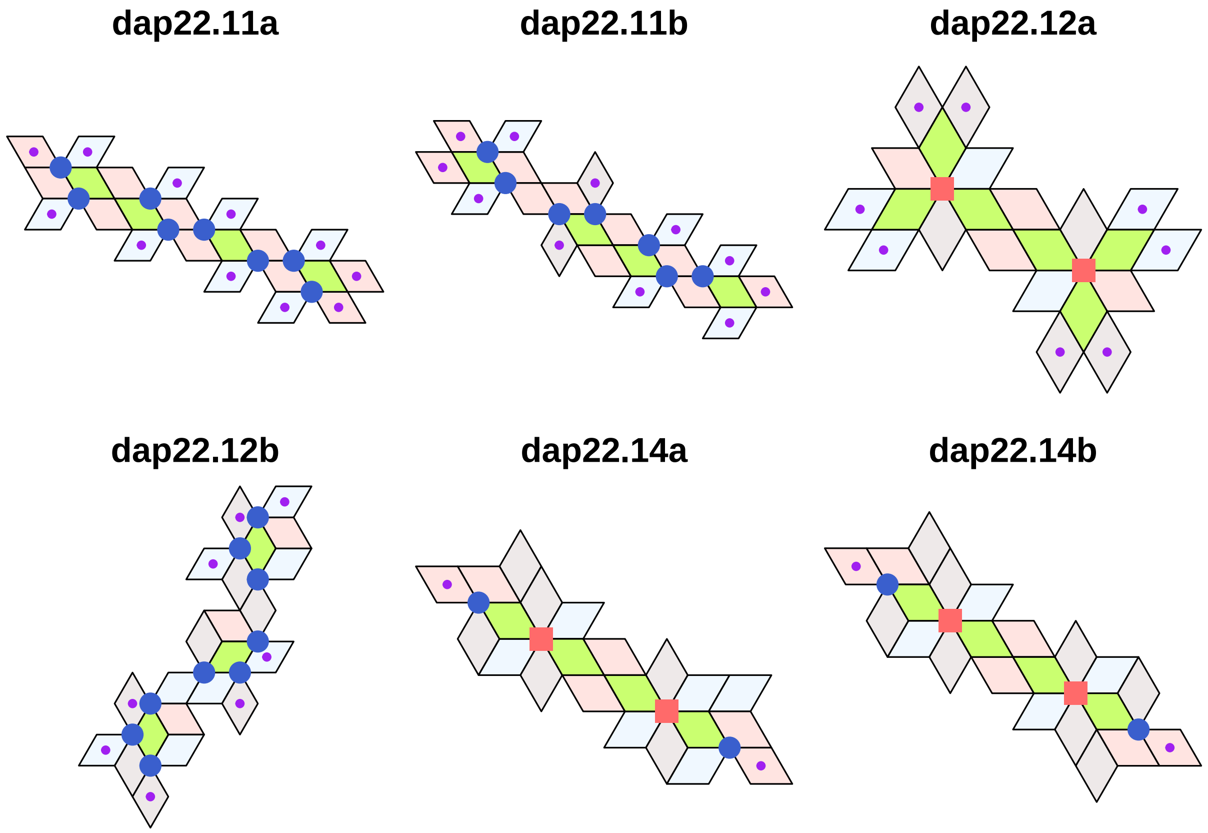


**Figure B16.** Tredoku tilings consisting of 22 tiles.

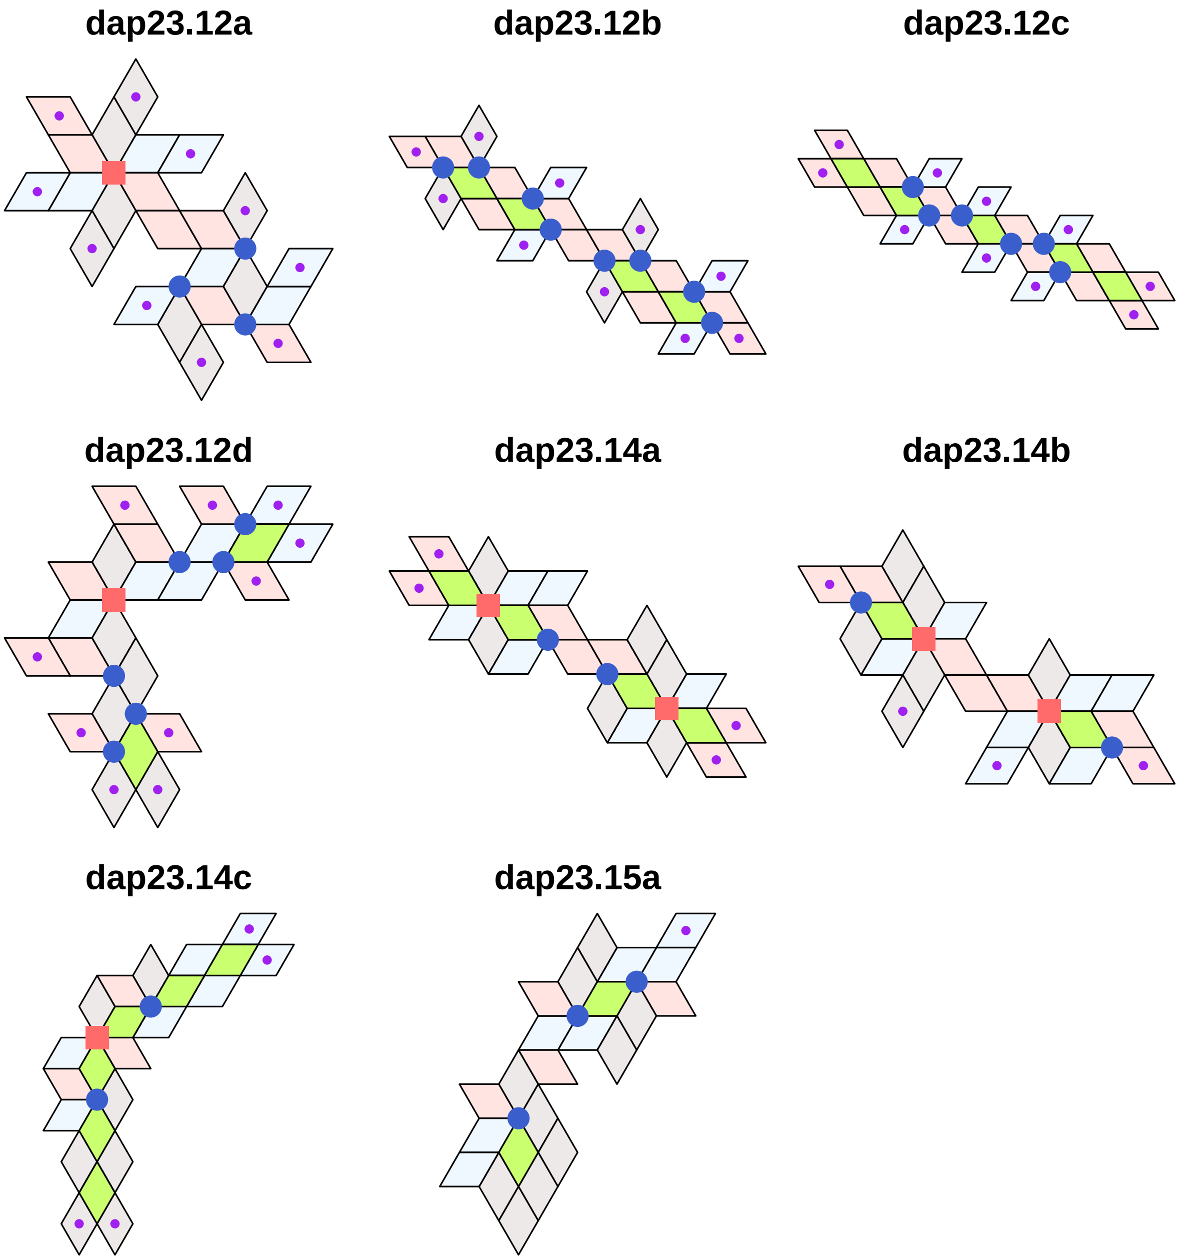


**Figure B17.** Tredoku tilings consisting of 23 tiles.

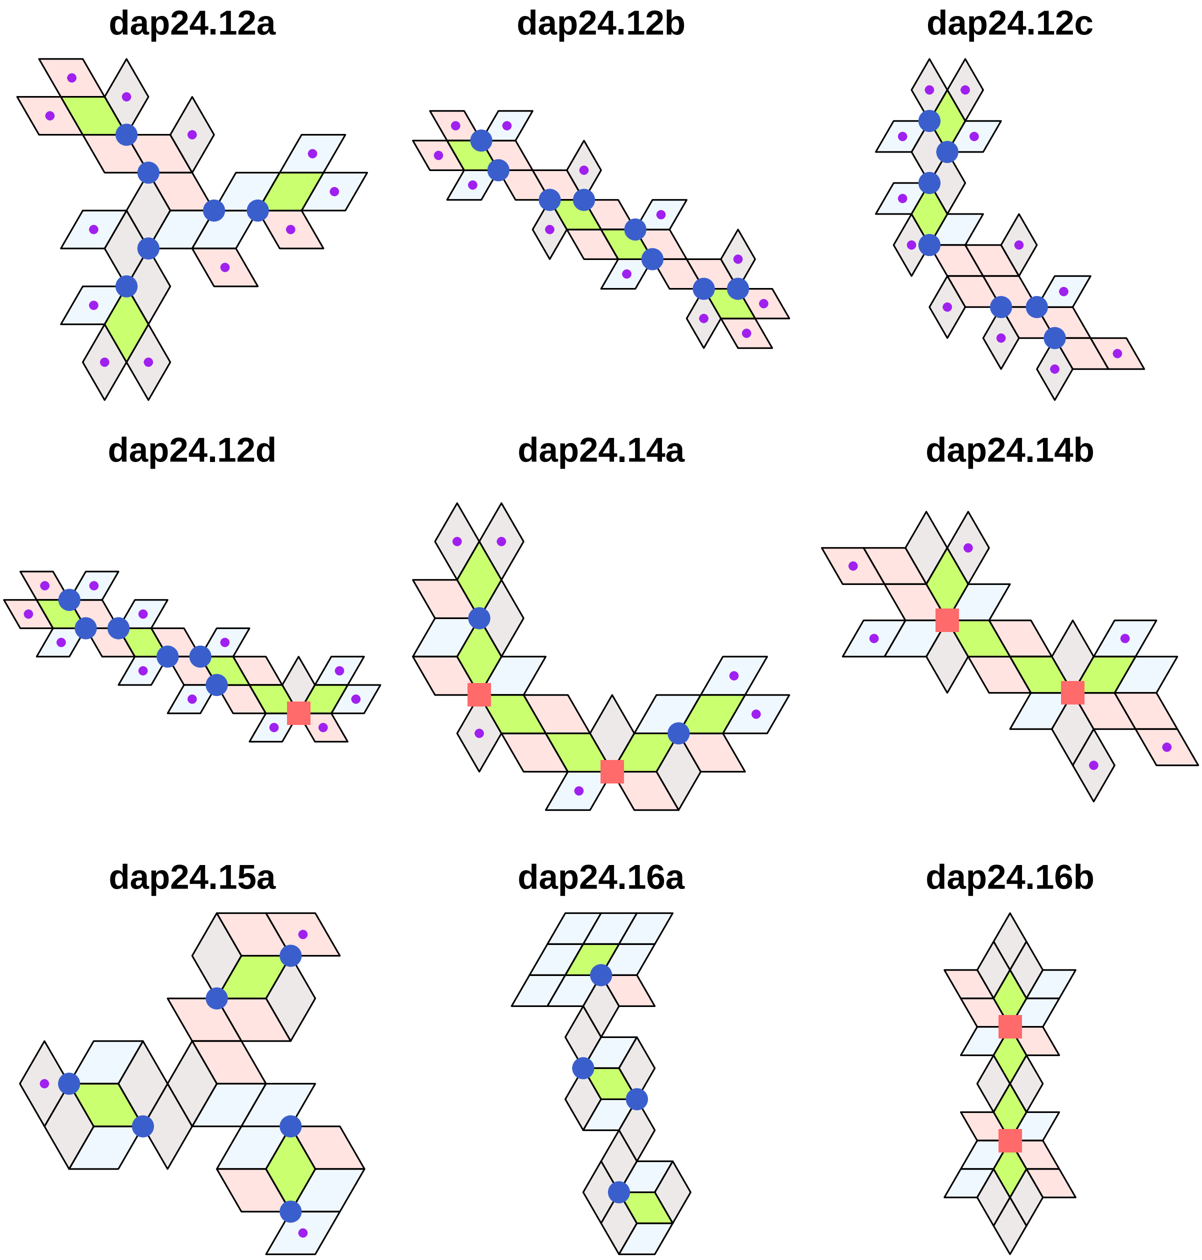


**Figure B18.** Tredoku tilings consisting of 24 tiles.

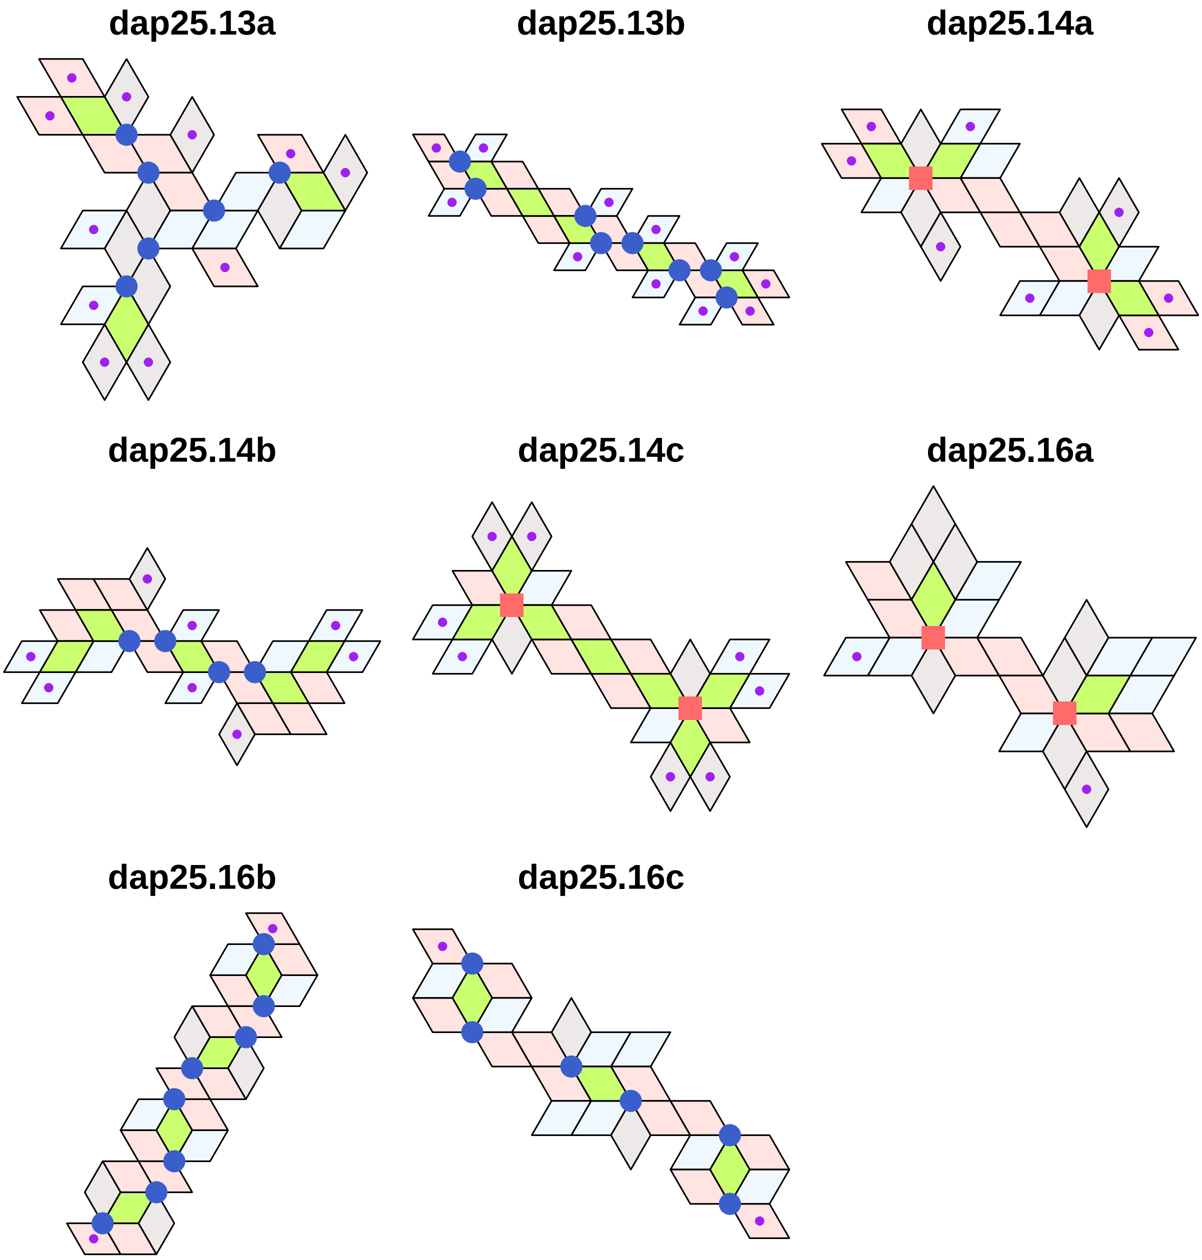


**Figure B19.** Tredoku tilings consisting of 25 tiles.

**dap26.13**

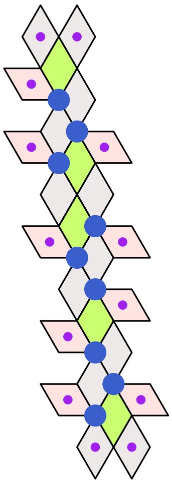

**dap28.14**

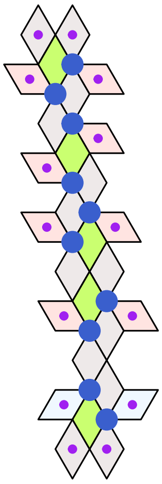

**dap30.15**

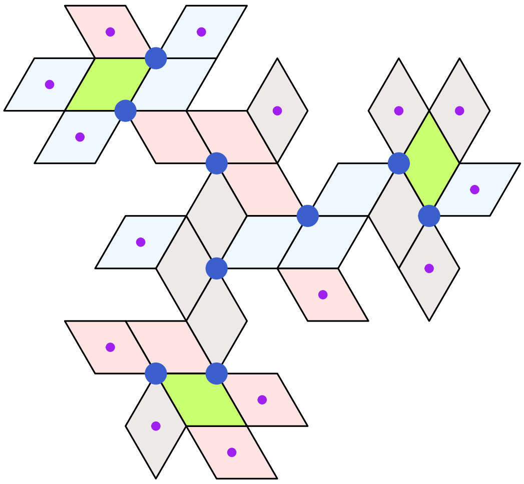

**dap32.16**

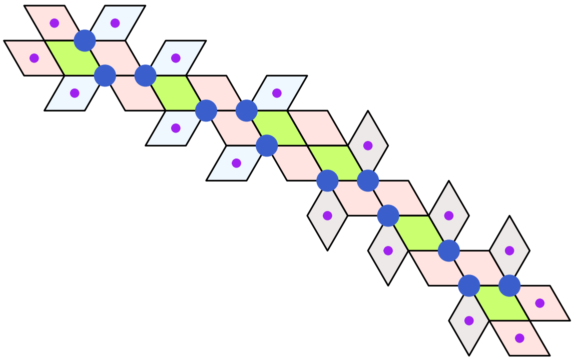

**dap34.17**

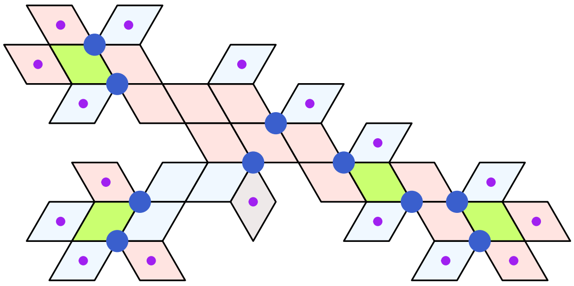

**dap36.18**

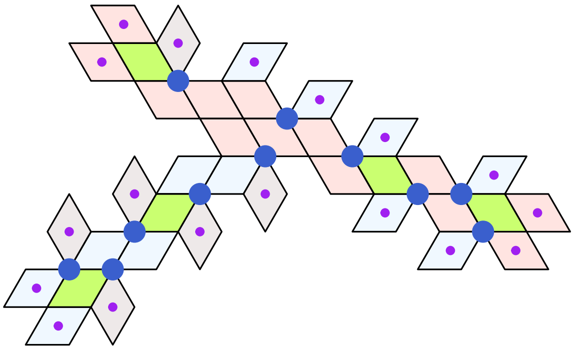

**Figure B20.** Tredoku tilings consisting of 26–36 tiles.

**dap38.19**

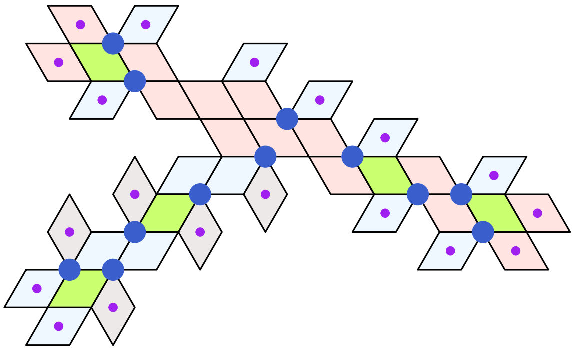

**dap41.21**

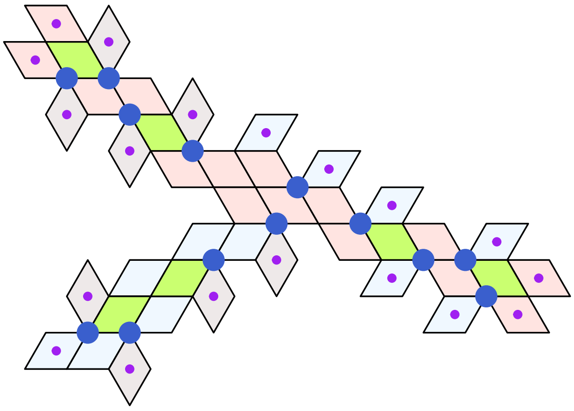

**dap42.21**

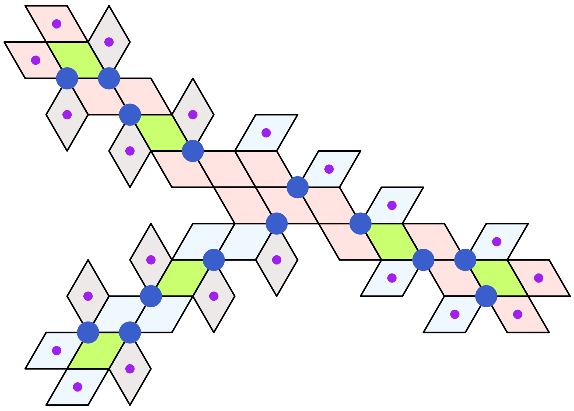

**Figure B21.** Tredoku tilings consisting of 38–42 tiles.
