# Supplementary material for: Professor Preece's tredoku tilings
Source: arXiv:2511.12680 ancillary file (2025-11-16)
Supplement: Supplementary file 3 [file Appendix_C.pdf]

## Professor Preece's Tredoku Tilings

## Appendix C - Quadridoku tilings

This appendix shows the quadridoku tilings that appear in Donald's notes.

For quadridoku tilings, Donald used different annotations to those that he employed for tredoku tilings. Tiles that are highlighted in orange indicate the potential for double merging, whilst runs of four tiles that are highlighted in green indicate the potential for four merging (see Section 7.1 in the paper).

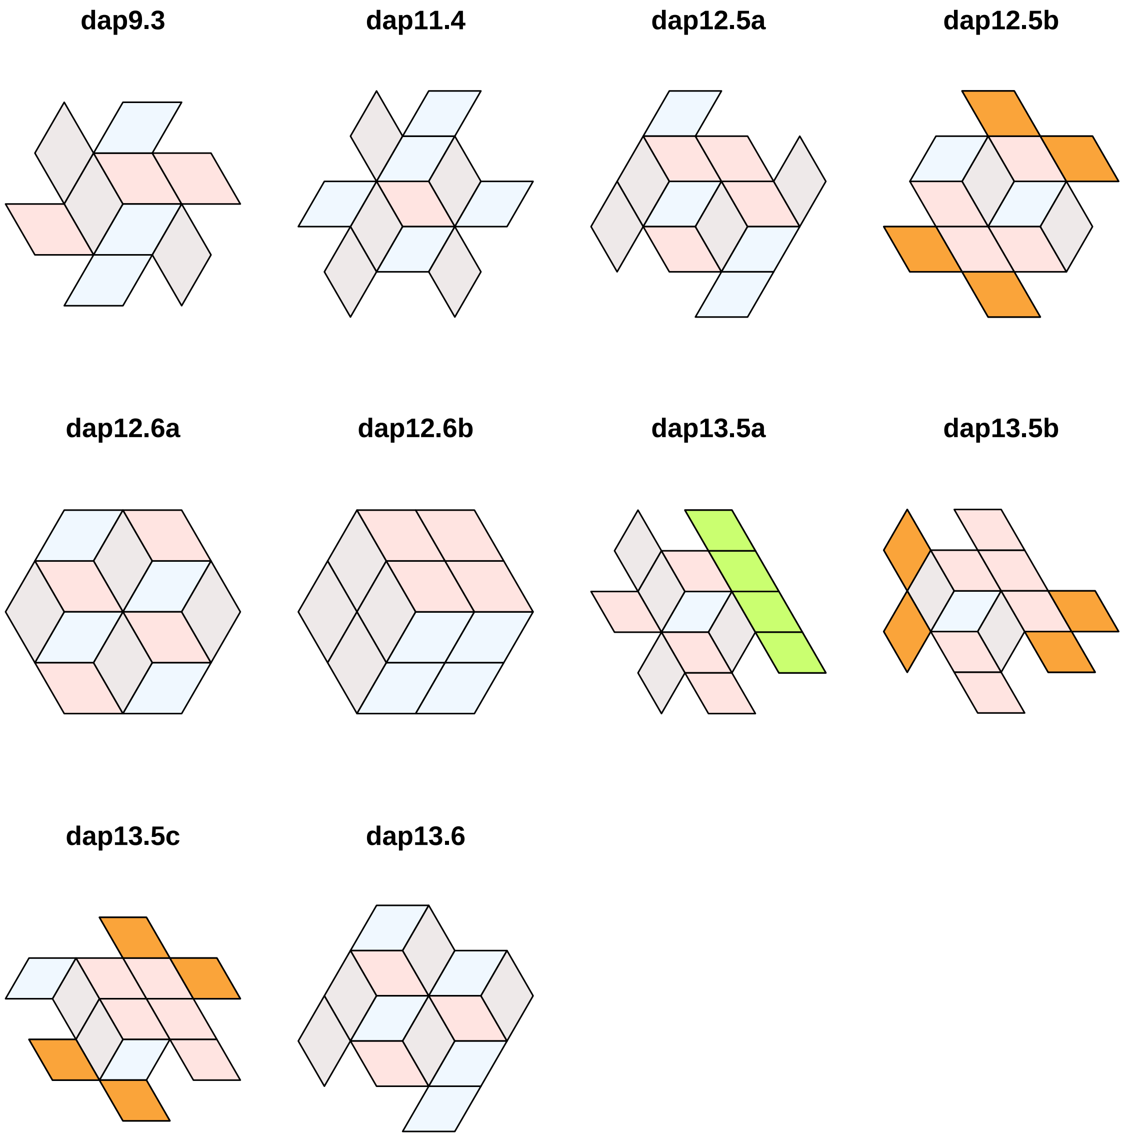


**Figure C1.** Quadridoku tilings consisting of 9–13 tiles.

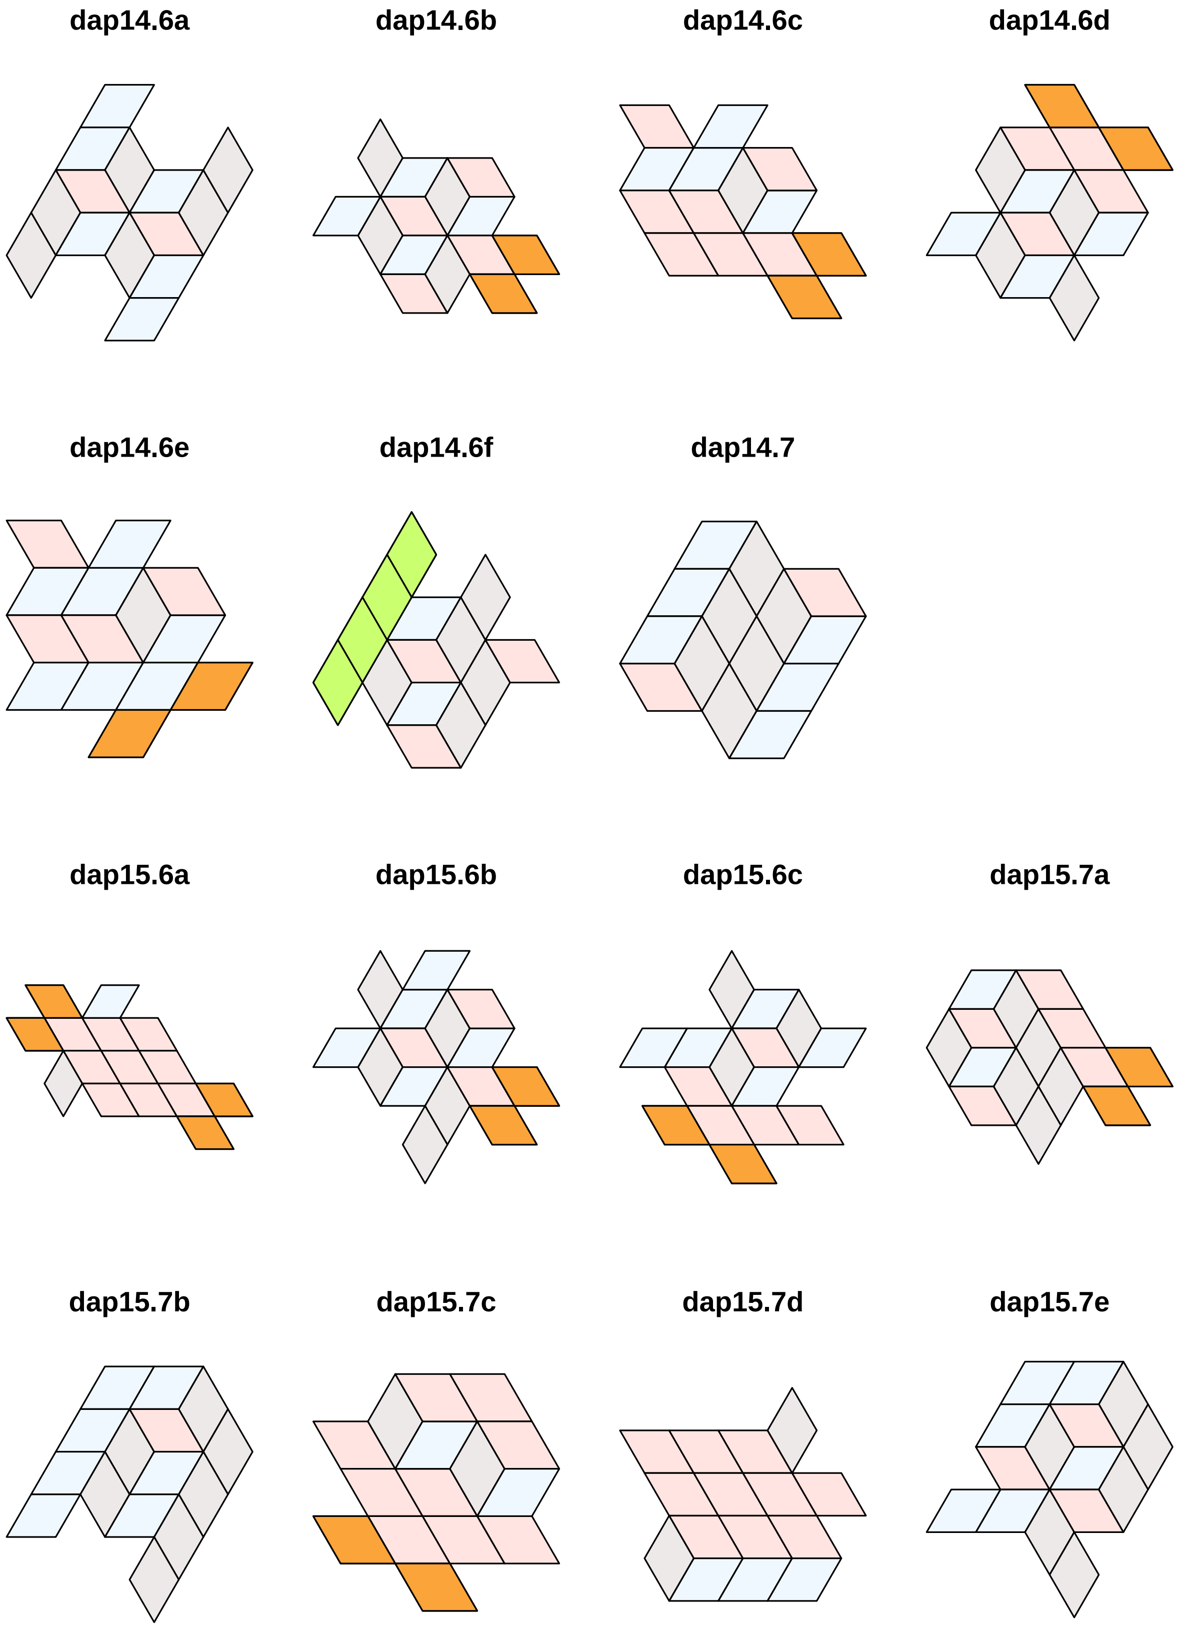


**Figure C2.** Quadridoku tilings consisting of 14 or 15 tiles.

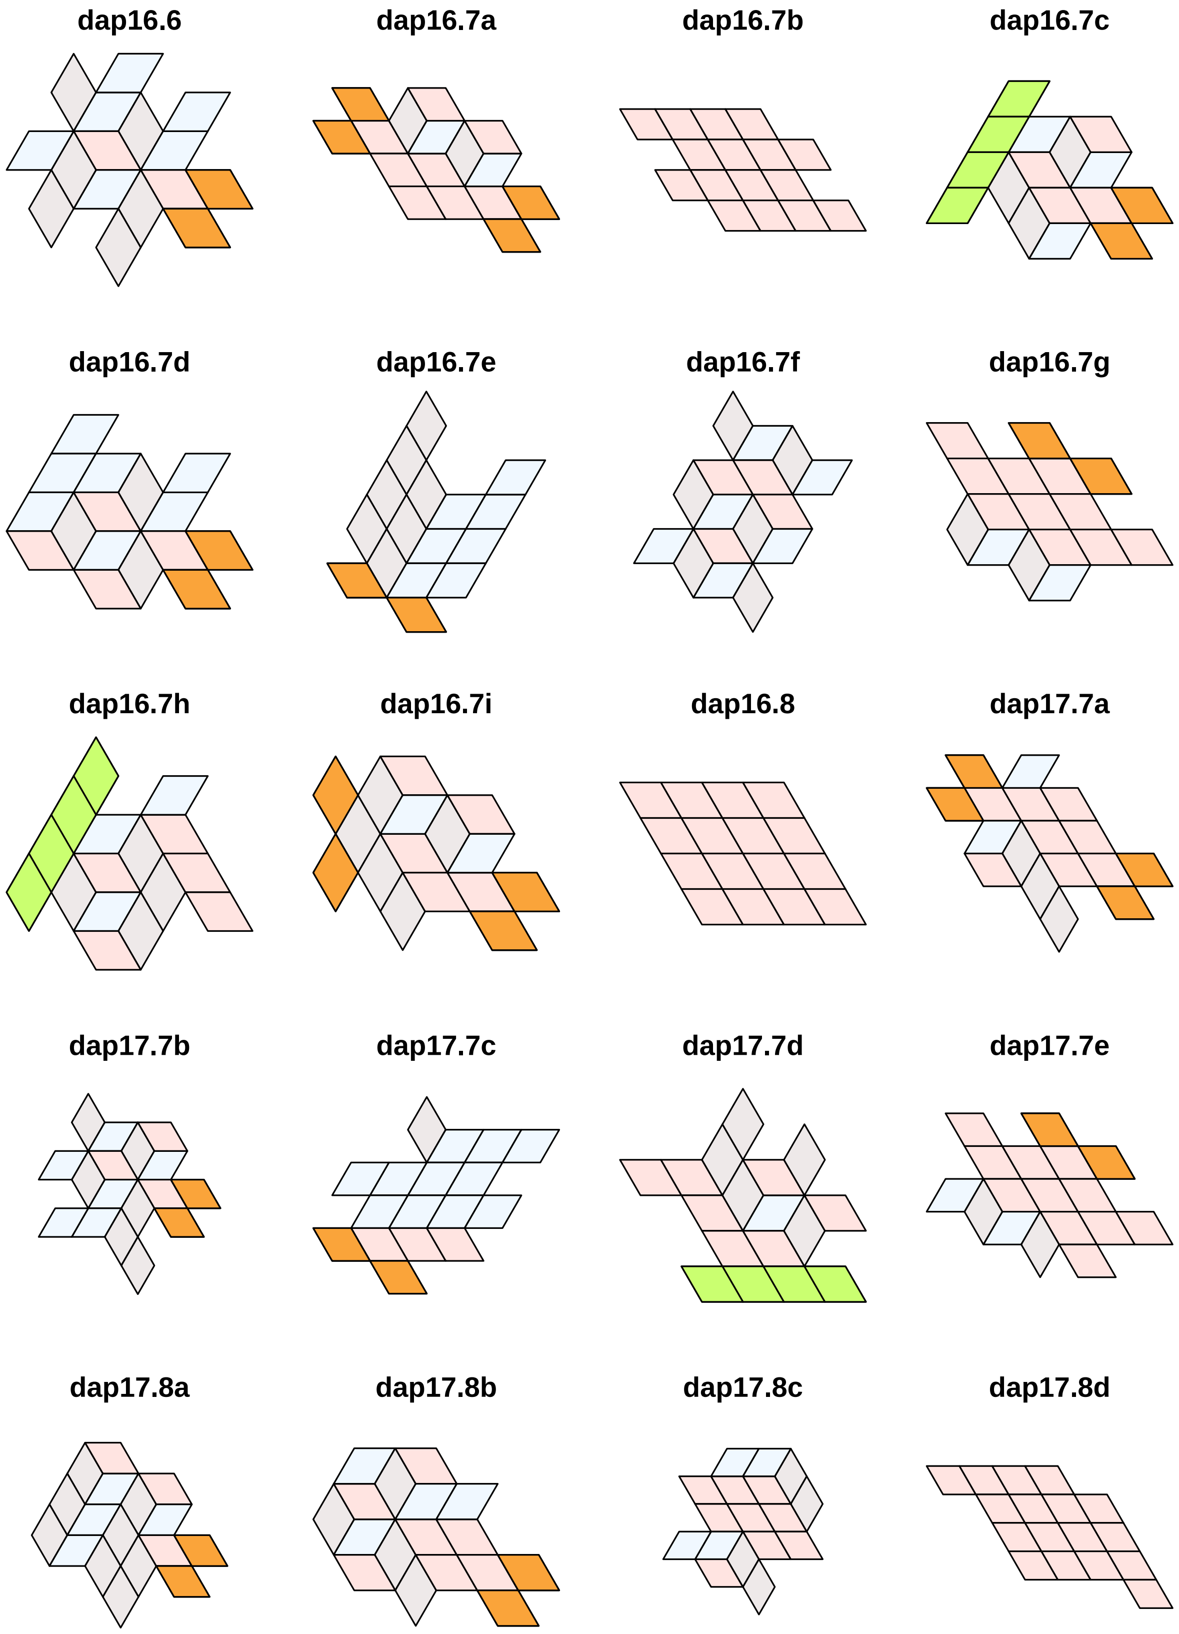


**Figure C3.** Quadridoku tilings consisting of 16 or 17 tiles.

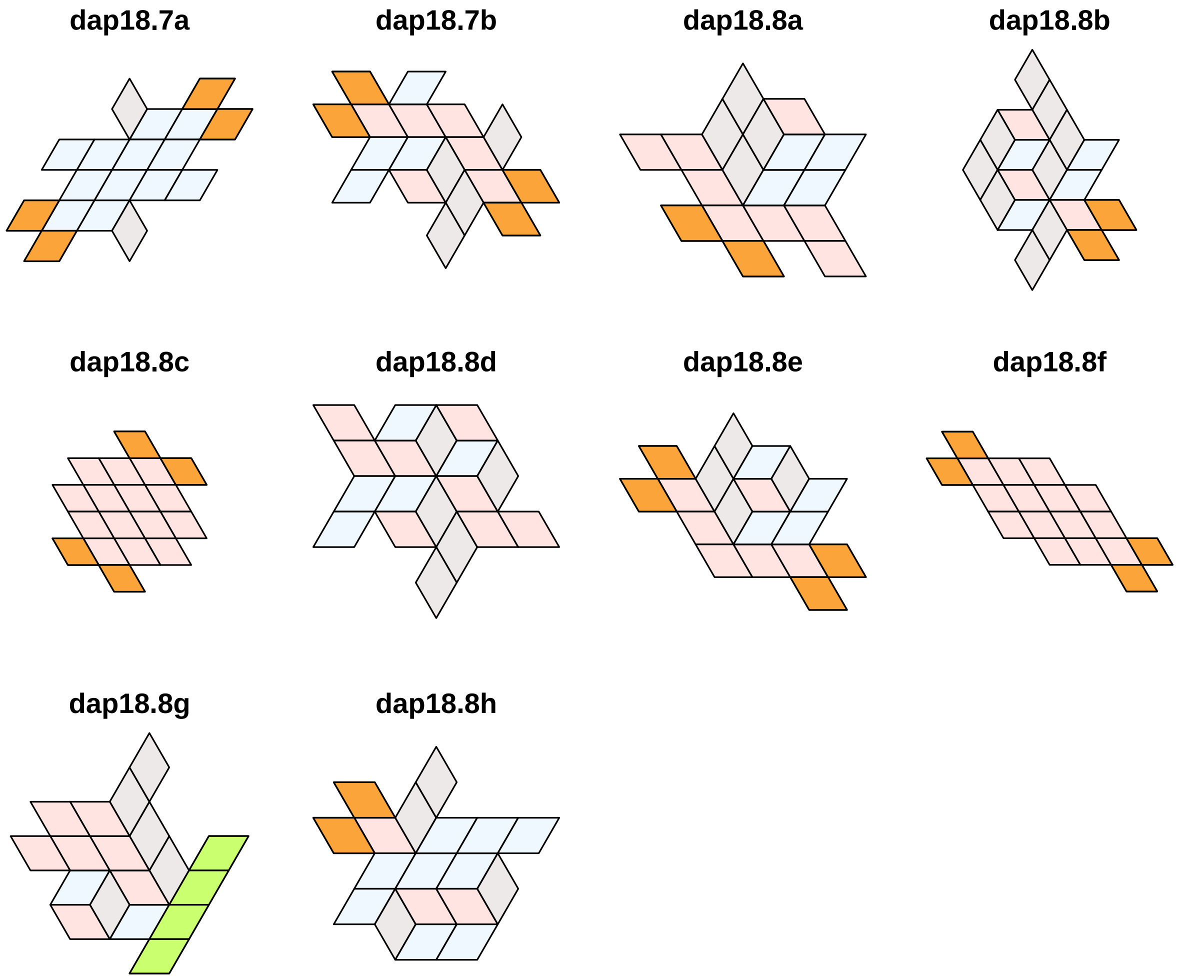


**Figure C4.** Quadridoku tilings consisting of 18 tiles.

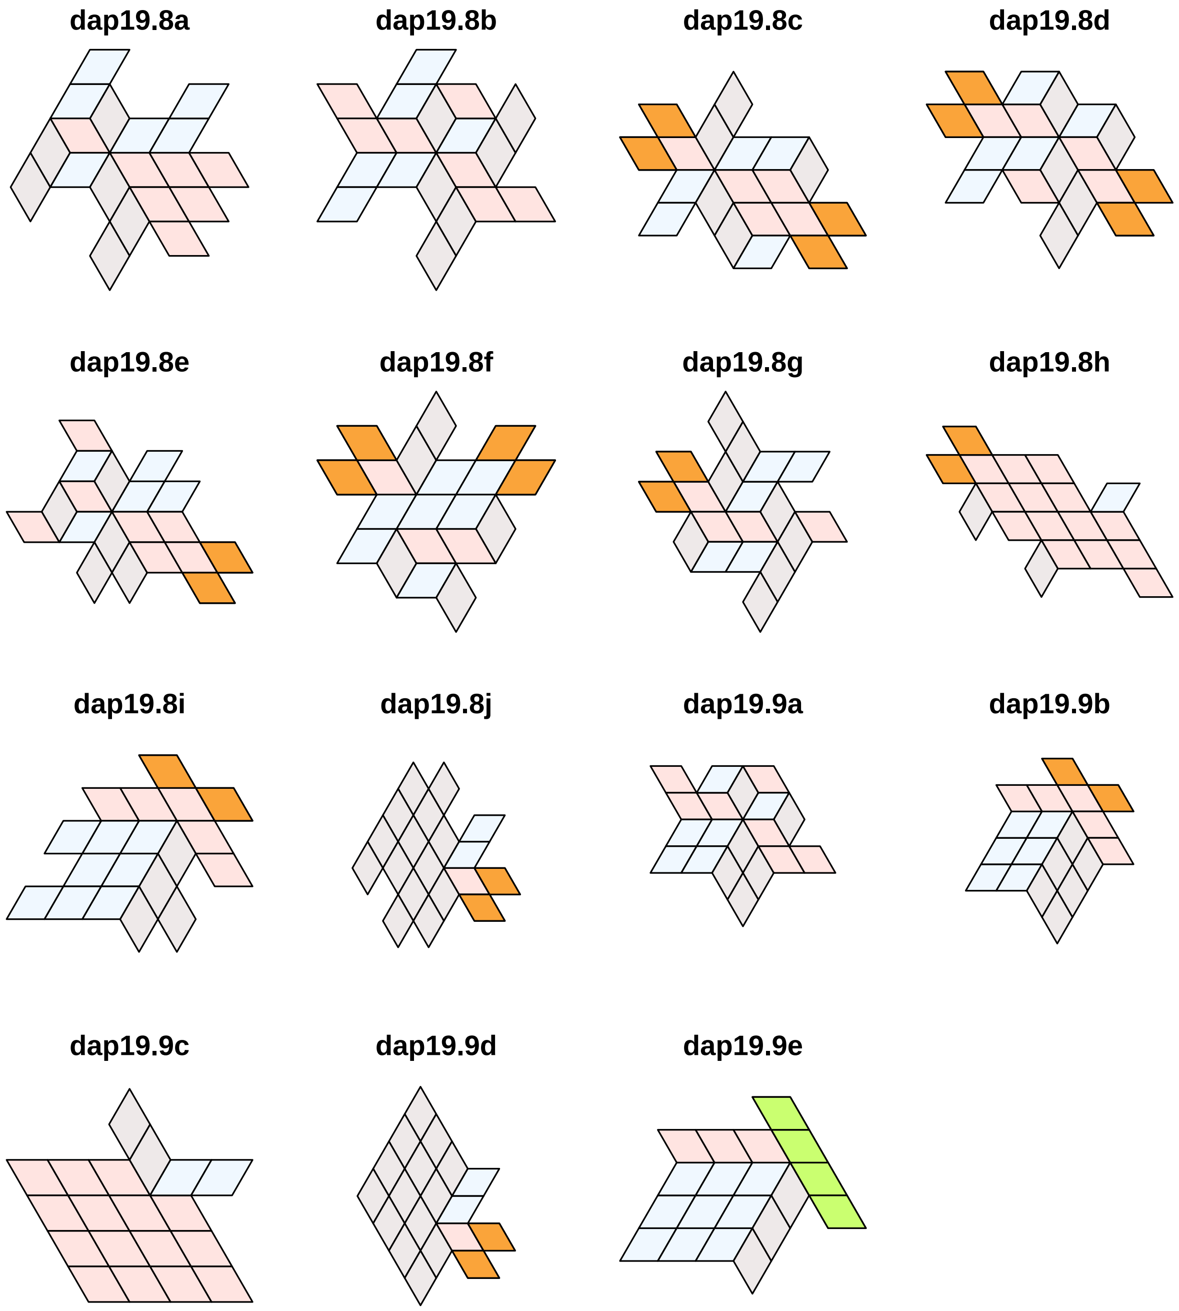


**Figure C5.** Quadridoku tilings consisting of 19 tiles.

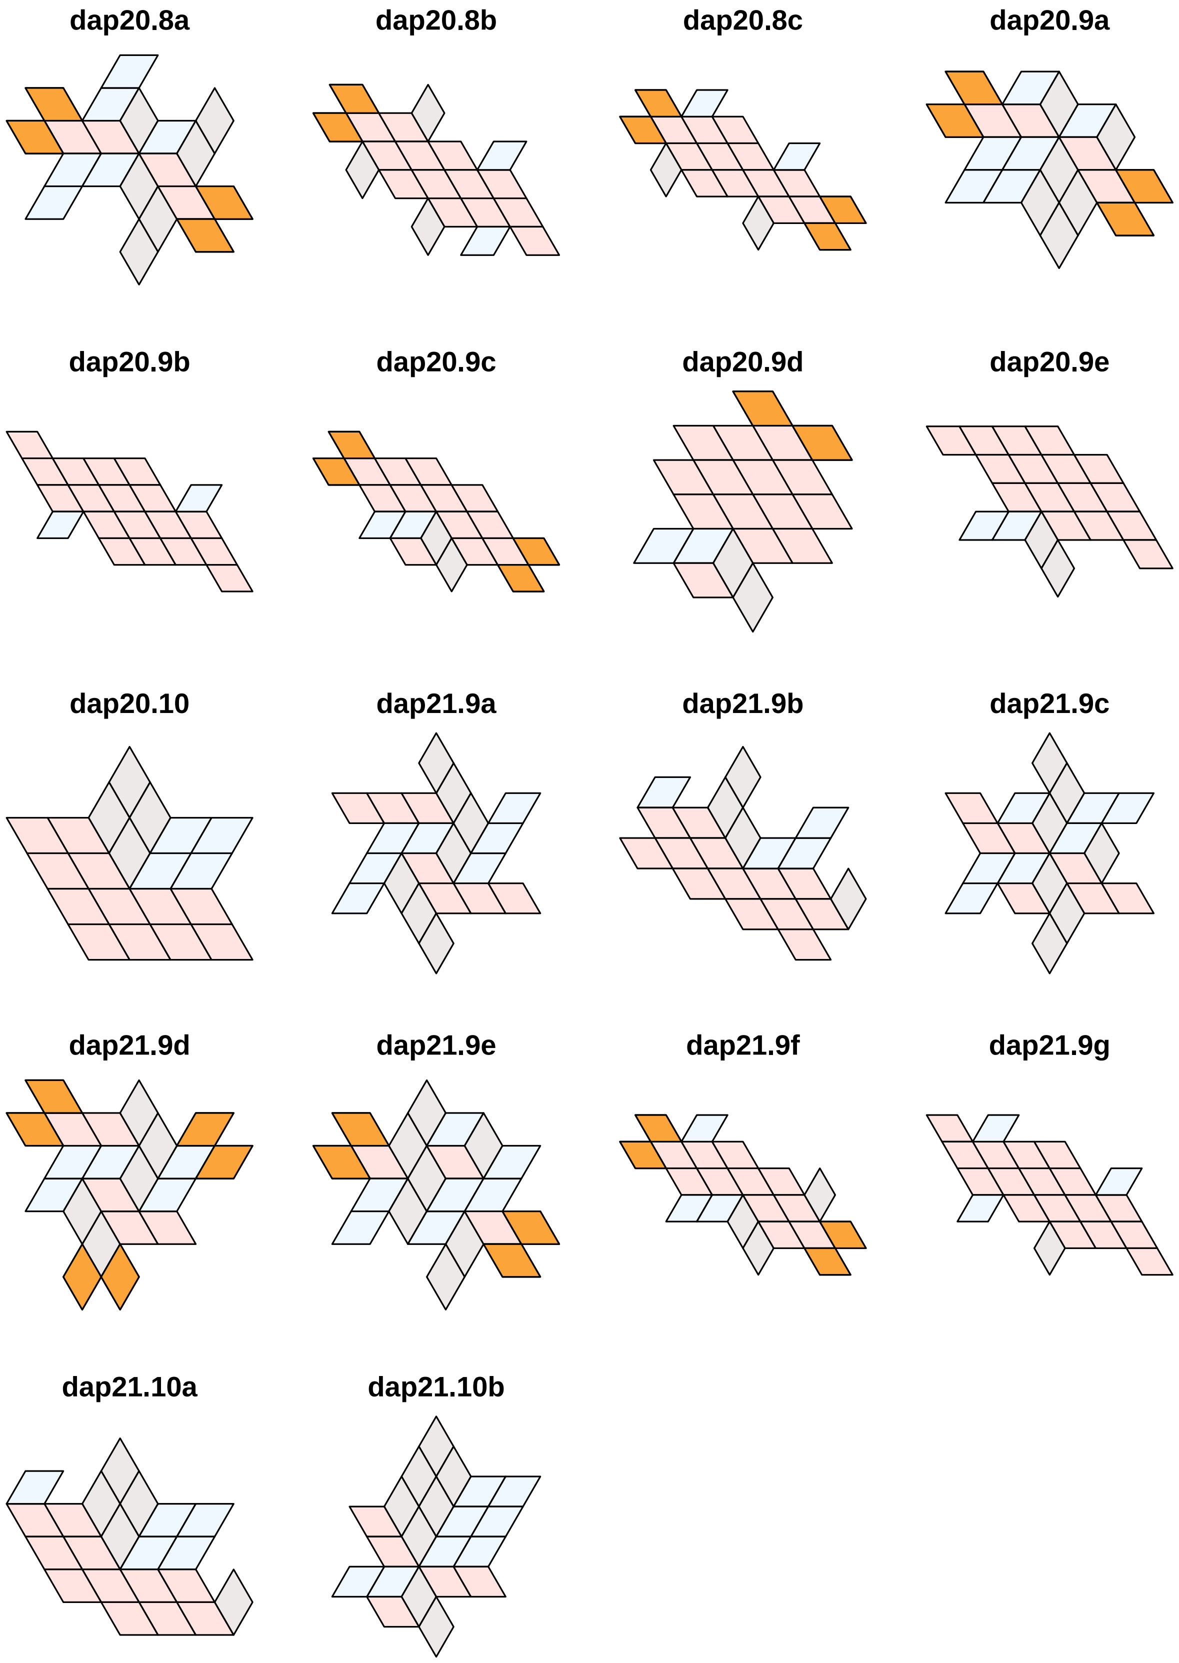


**Figure C6.** Quadridoku tilings consisting of 20 or 21 tiles.

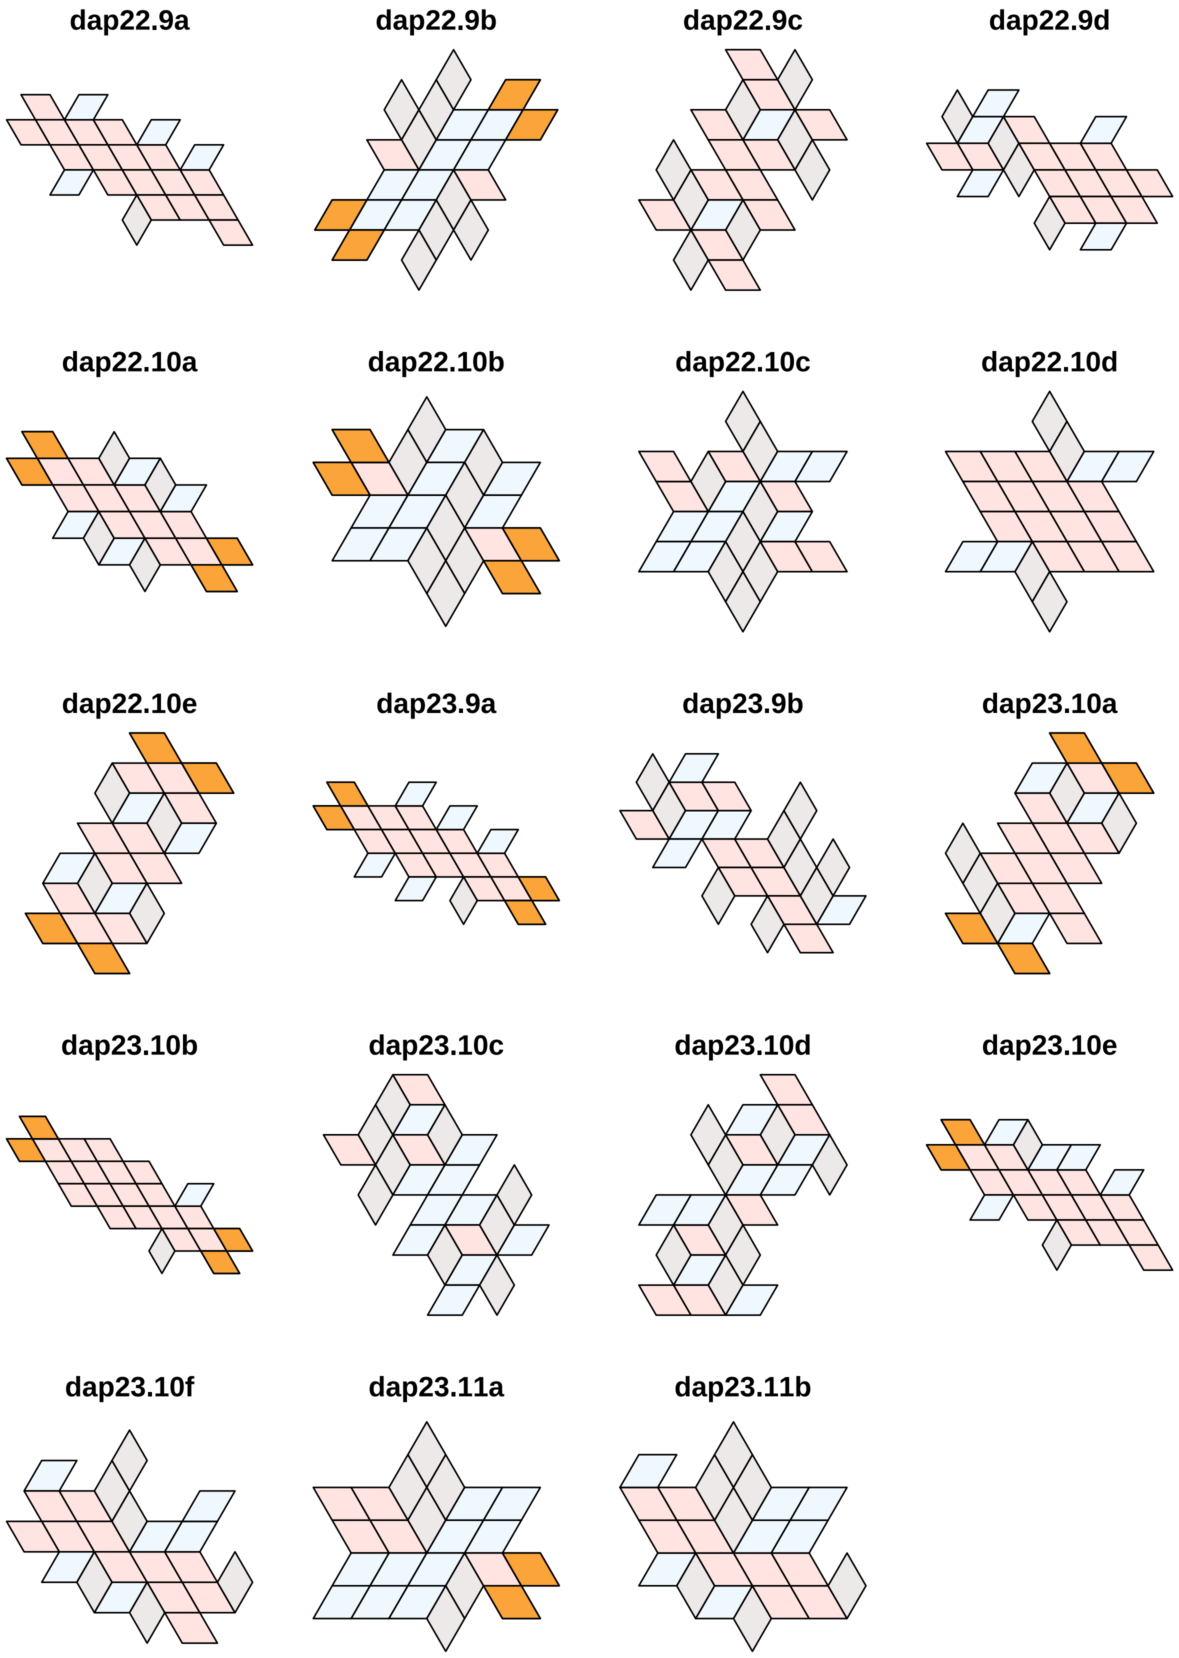


**Figure C7.** Quadridoku tilings consisting of 22 or 23 tiles.

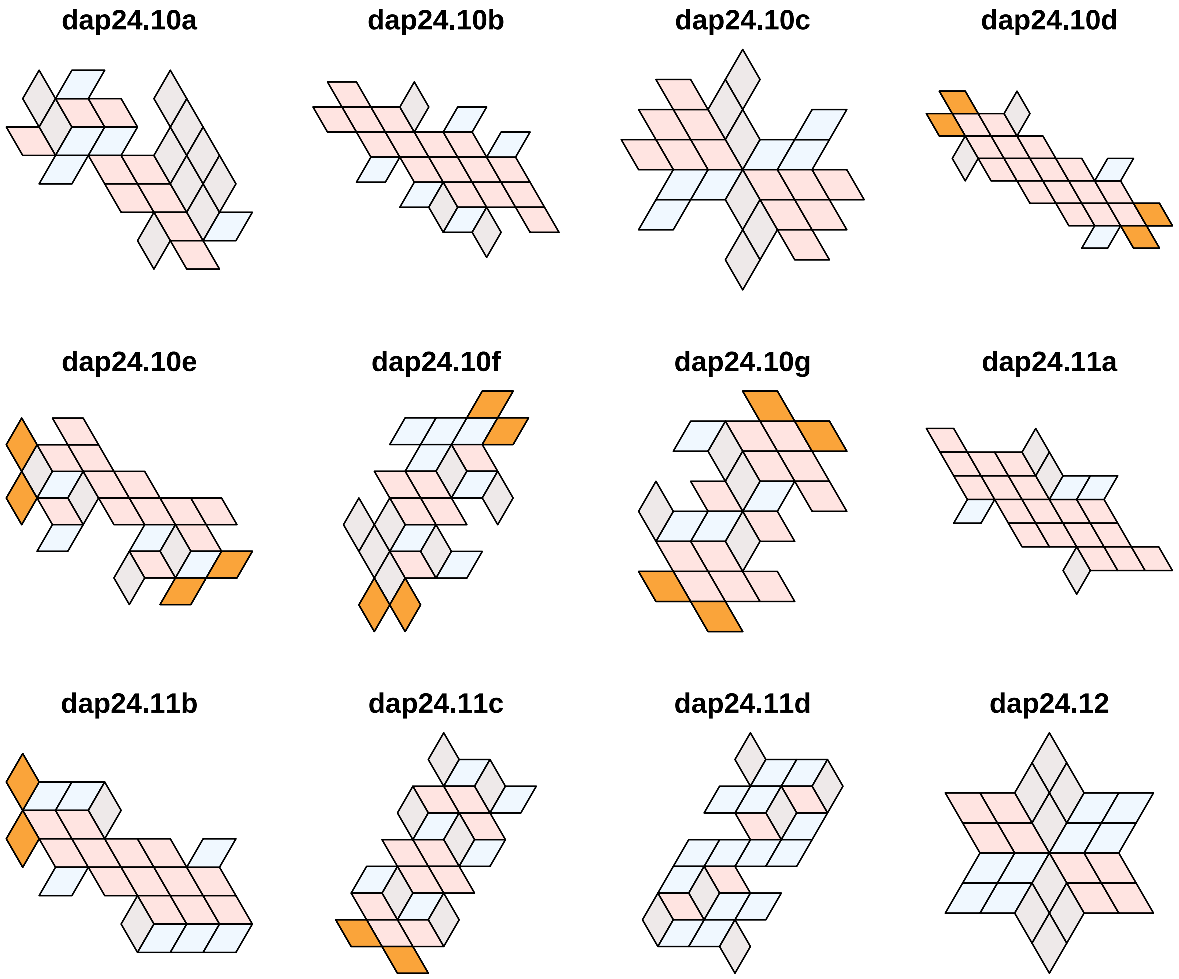


**Figure C8.** Quadridoku tilings consisting of 24 tiles.

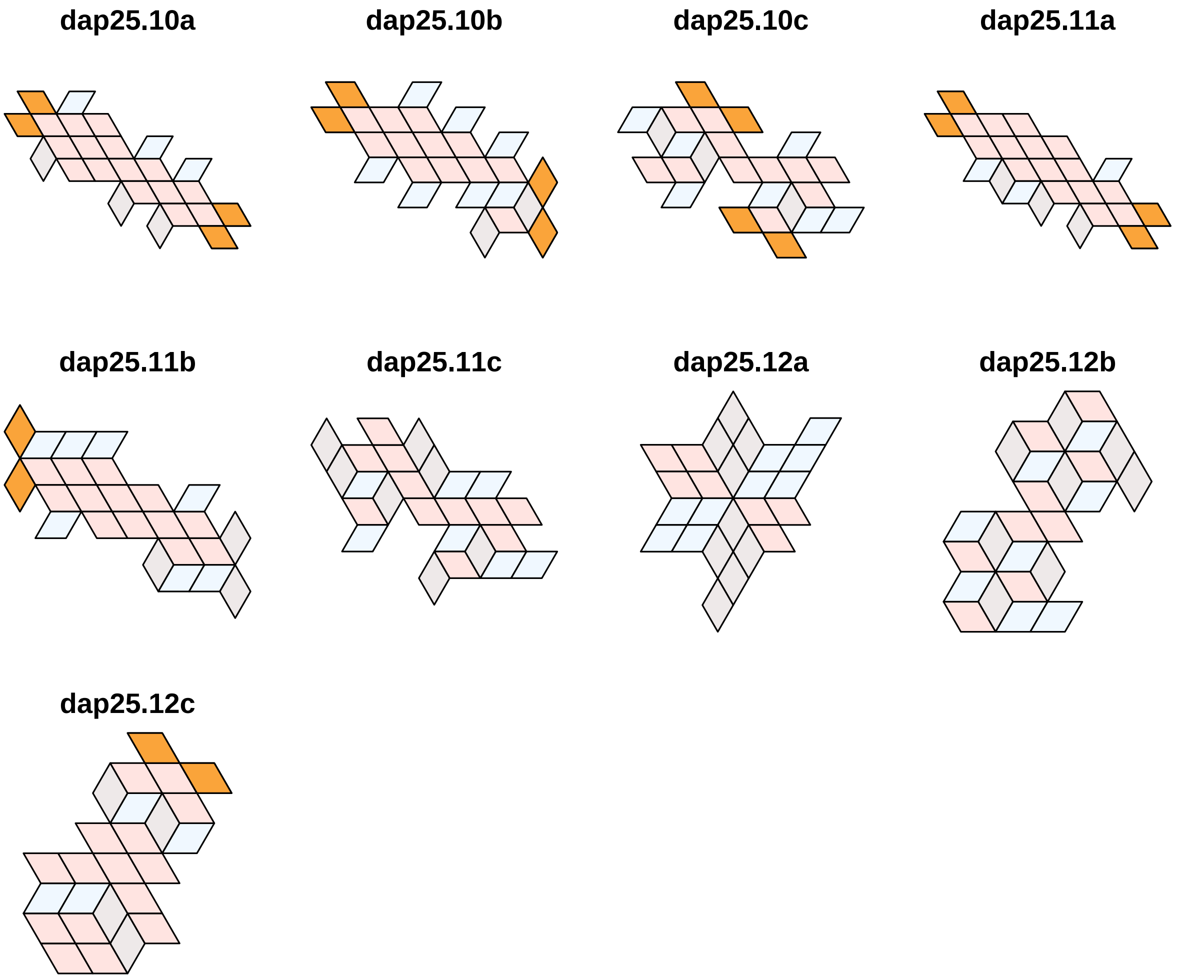


**Figure C9.** Quadridoku tilings consisting of 25 tiles.

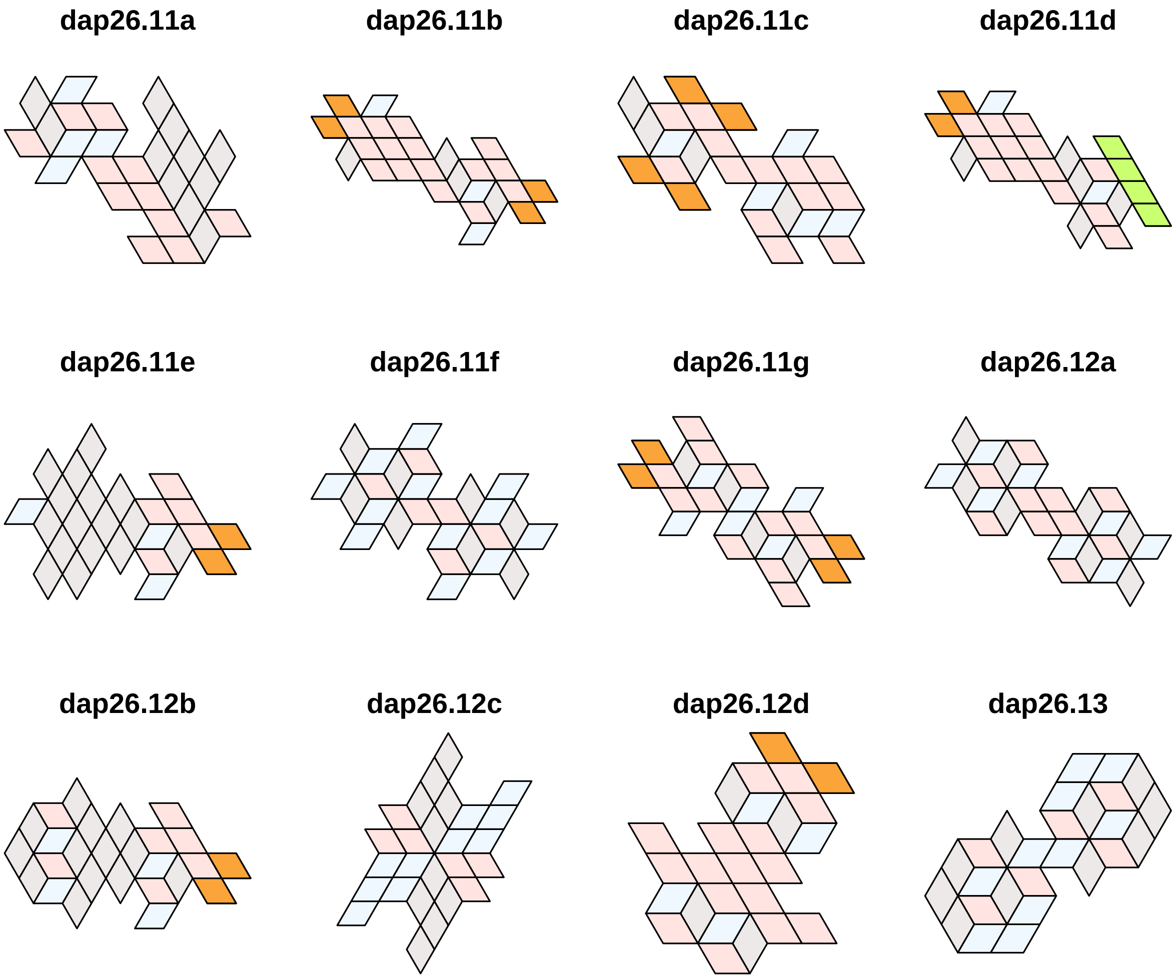


**Figure C10.** Quadridoku tilings consisting of 26 tiles.

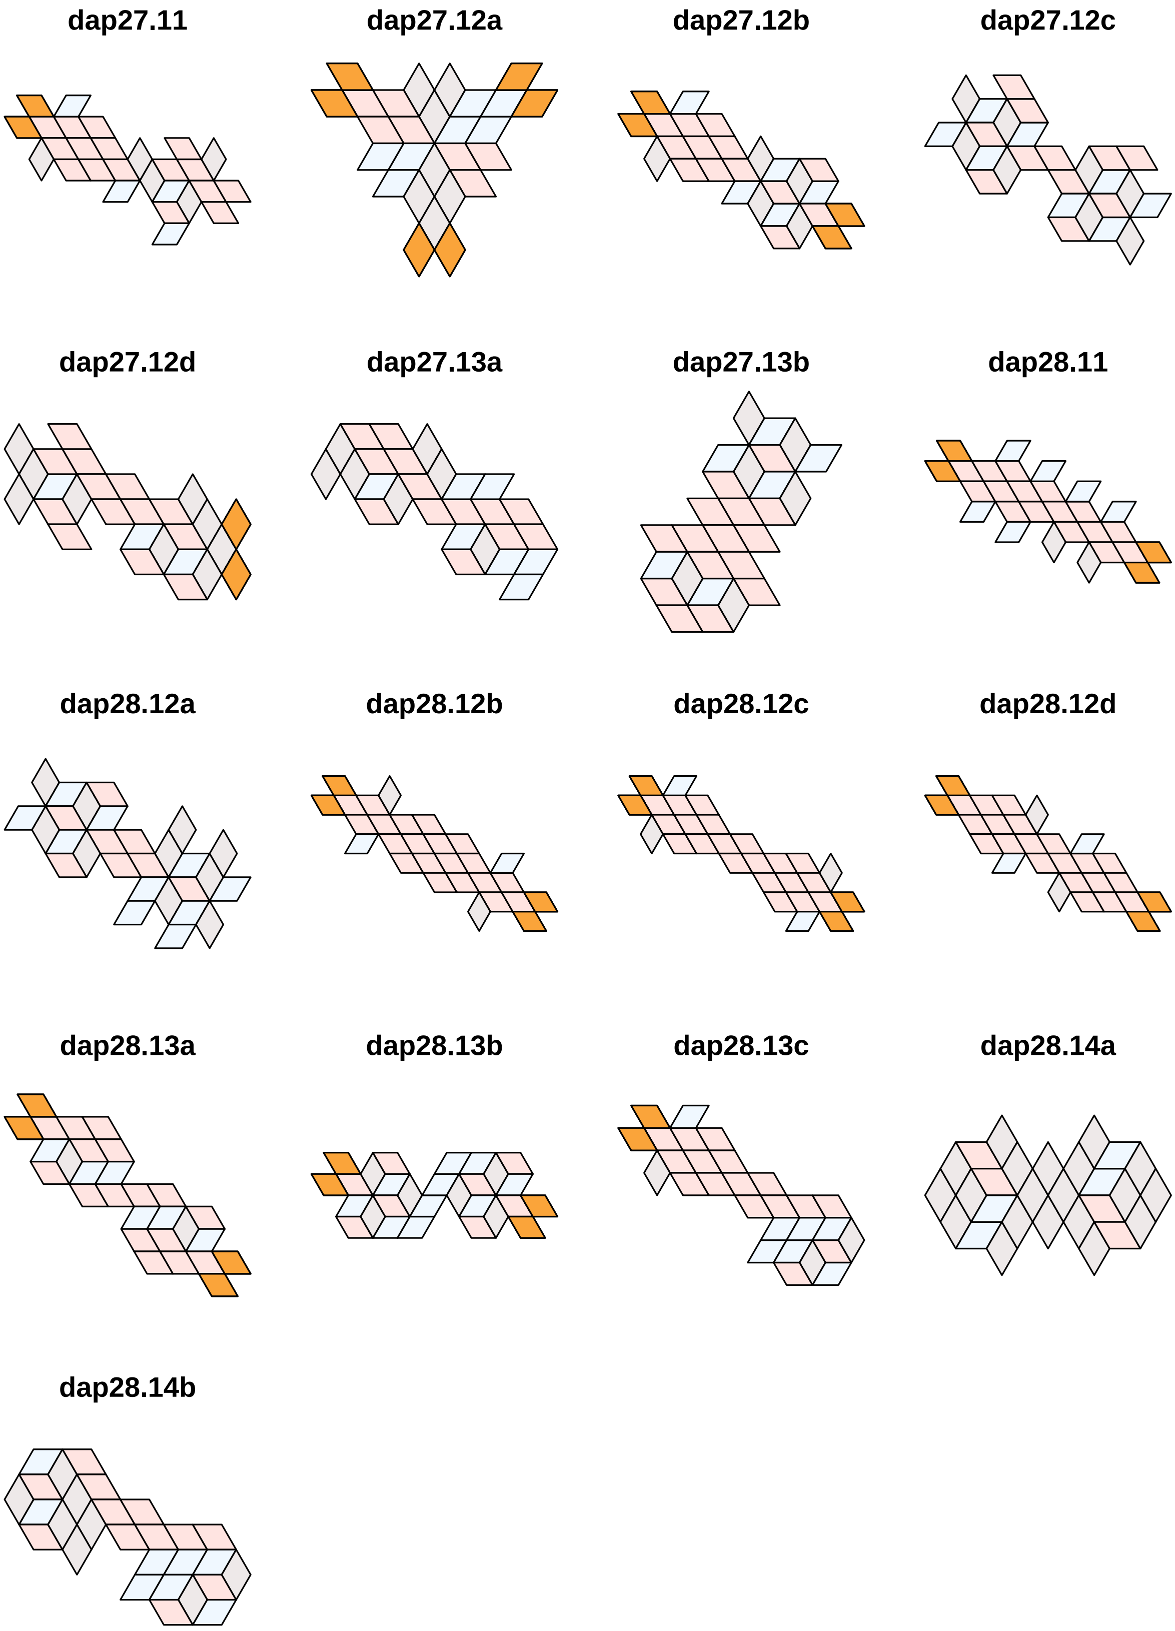


**Figure C11.** Quadridoku tilings consisting of 27 or 28 tiles.

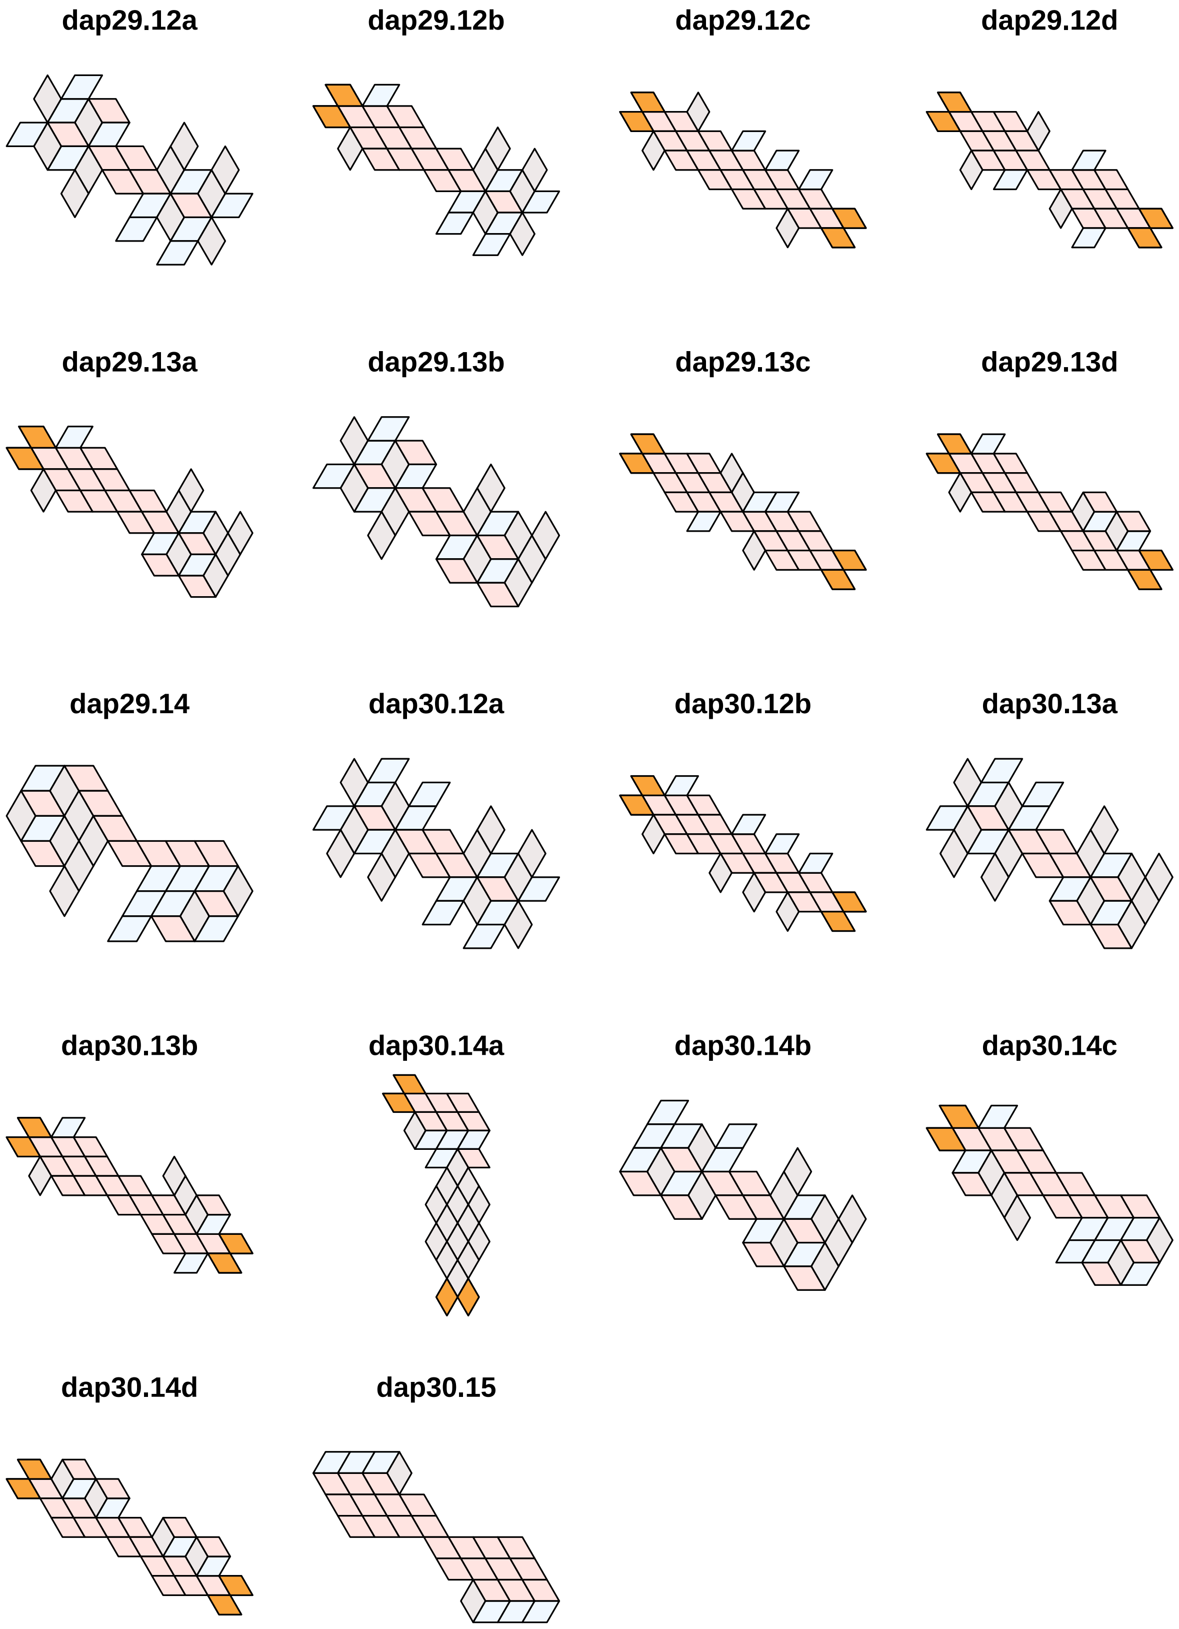


**Figure C12.** Quadridoku tilings consisting of 29 or 30 tiles.
