# Supplementary material for: Professor Preece's tredoku tilings
Source: arXiv:2511.12680 ancillary file (2025-11-16)
Supplement: Supplementary file 4 [file Appendix_D.pdf]

## Professor Preece's Tredoku Tilings

### Appendix D - Donald's quindoku tilings

This appendix shows the seventeen quindoku tilings that appear in Donald's notes.

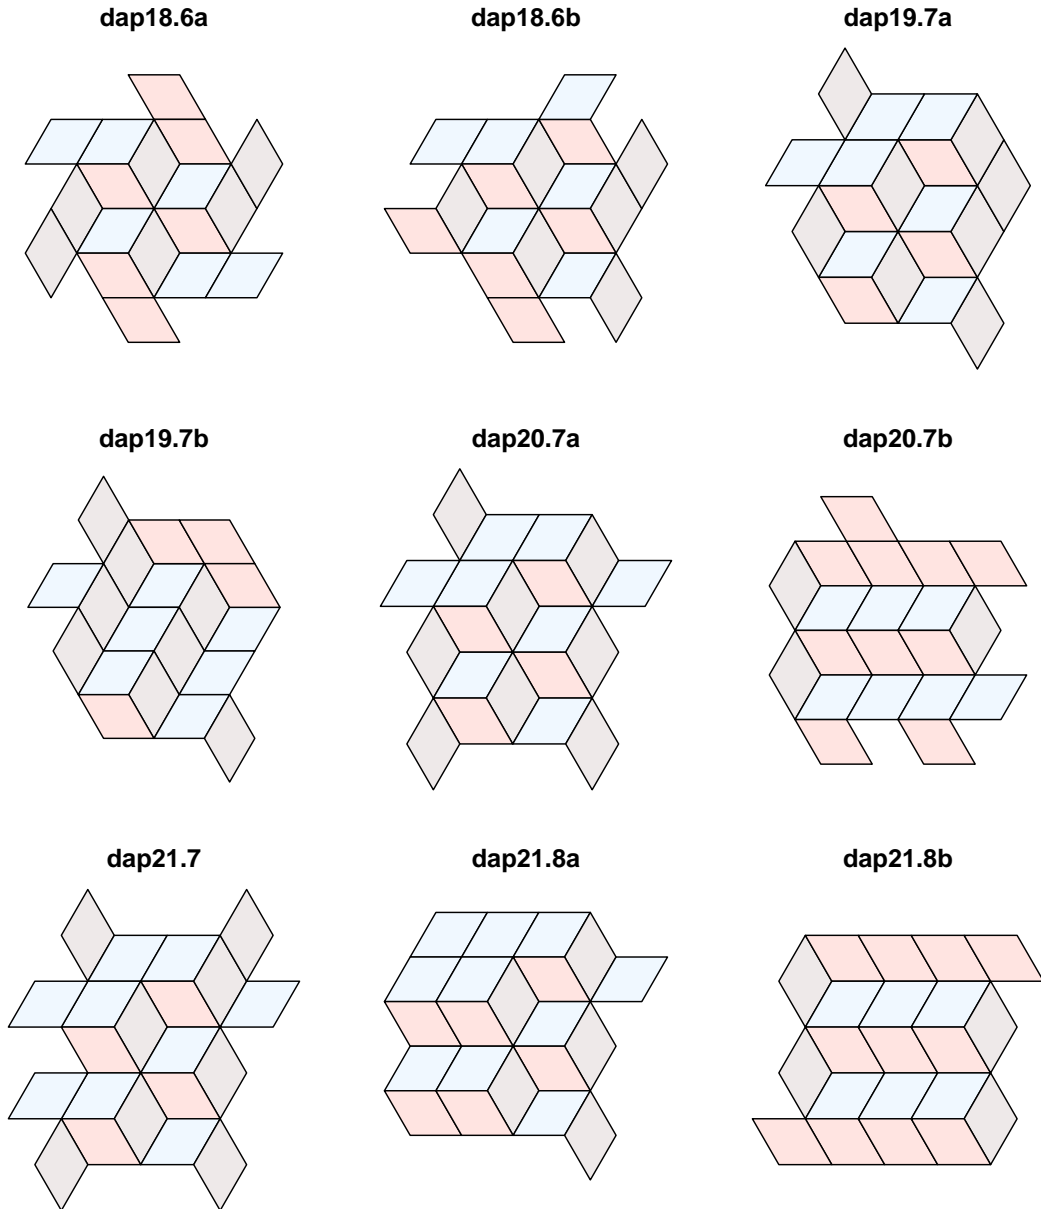

**Figure D1.** Quindoku tilings consisting of 18–21 tiles.

**dap22.8a**

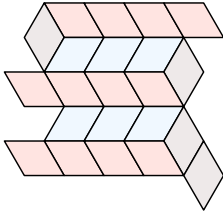

**dap22.8b**

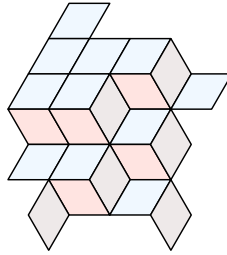

**dap23.8**

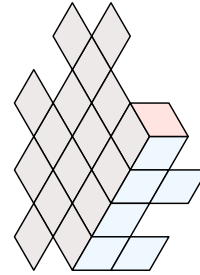

**dap23.9**

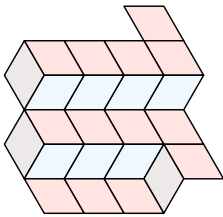

**dap24.8**

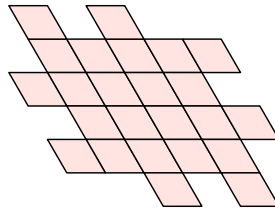

**dap24.9**

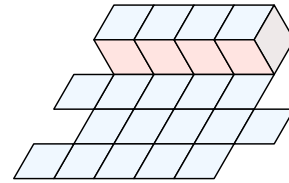

**dap25.9**

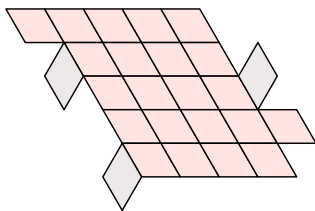

**dap25.10**

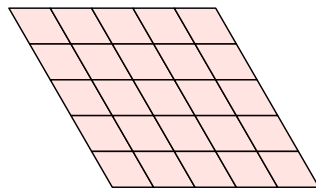

**Figure D2.** Quindoku tilings consisting of 22–25 tiles.
